# Supplementary material for: Network Methods for Pathway Analysis of Genomic Data
Source: arXiv:1411.1993 source file (2014-11-07)

# GSE13876 data

-log10(p) vals by method

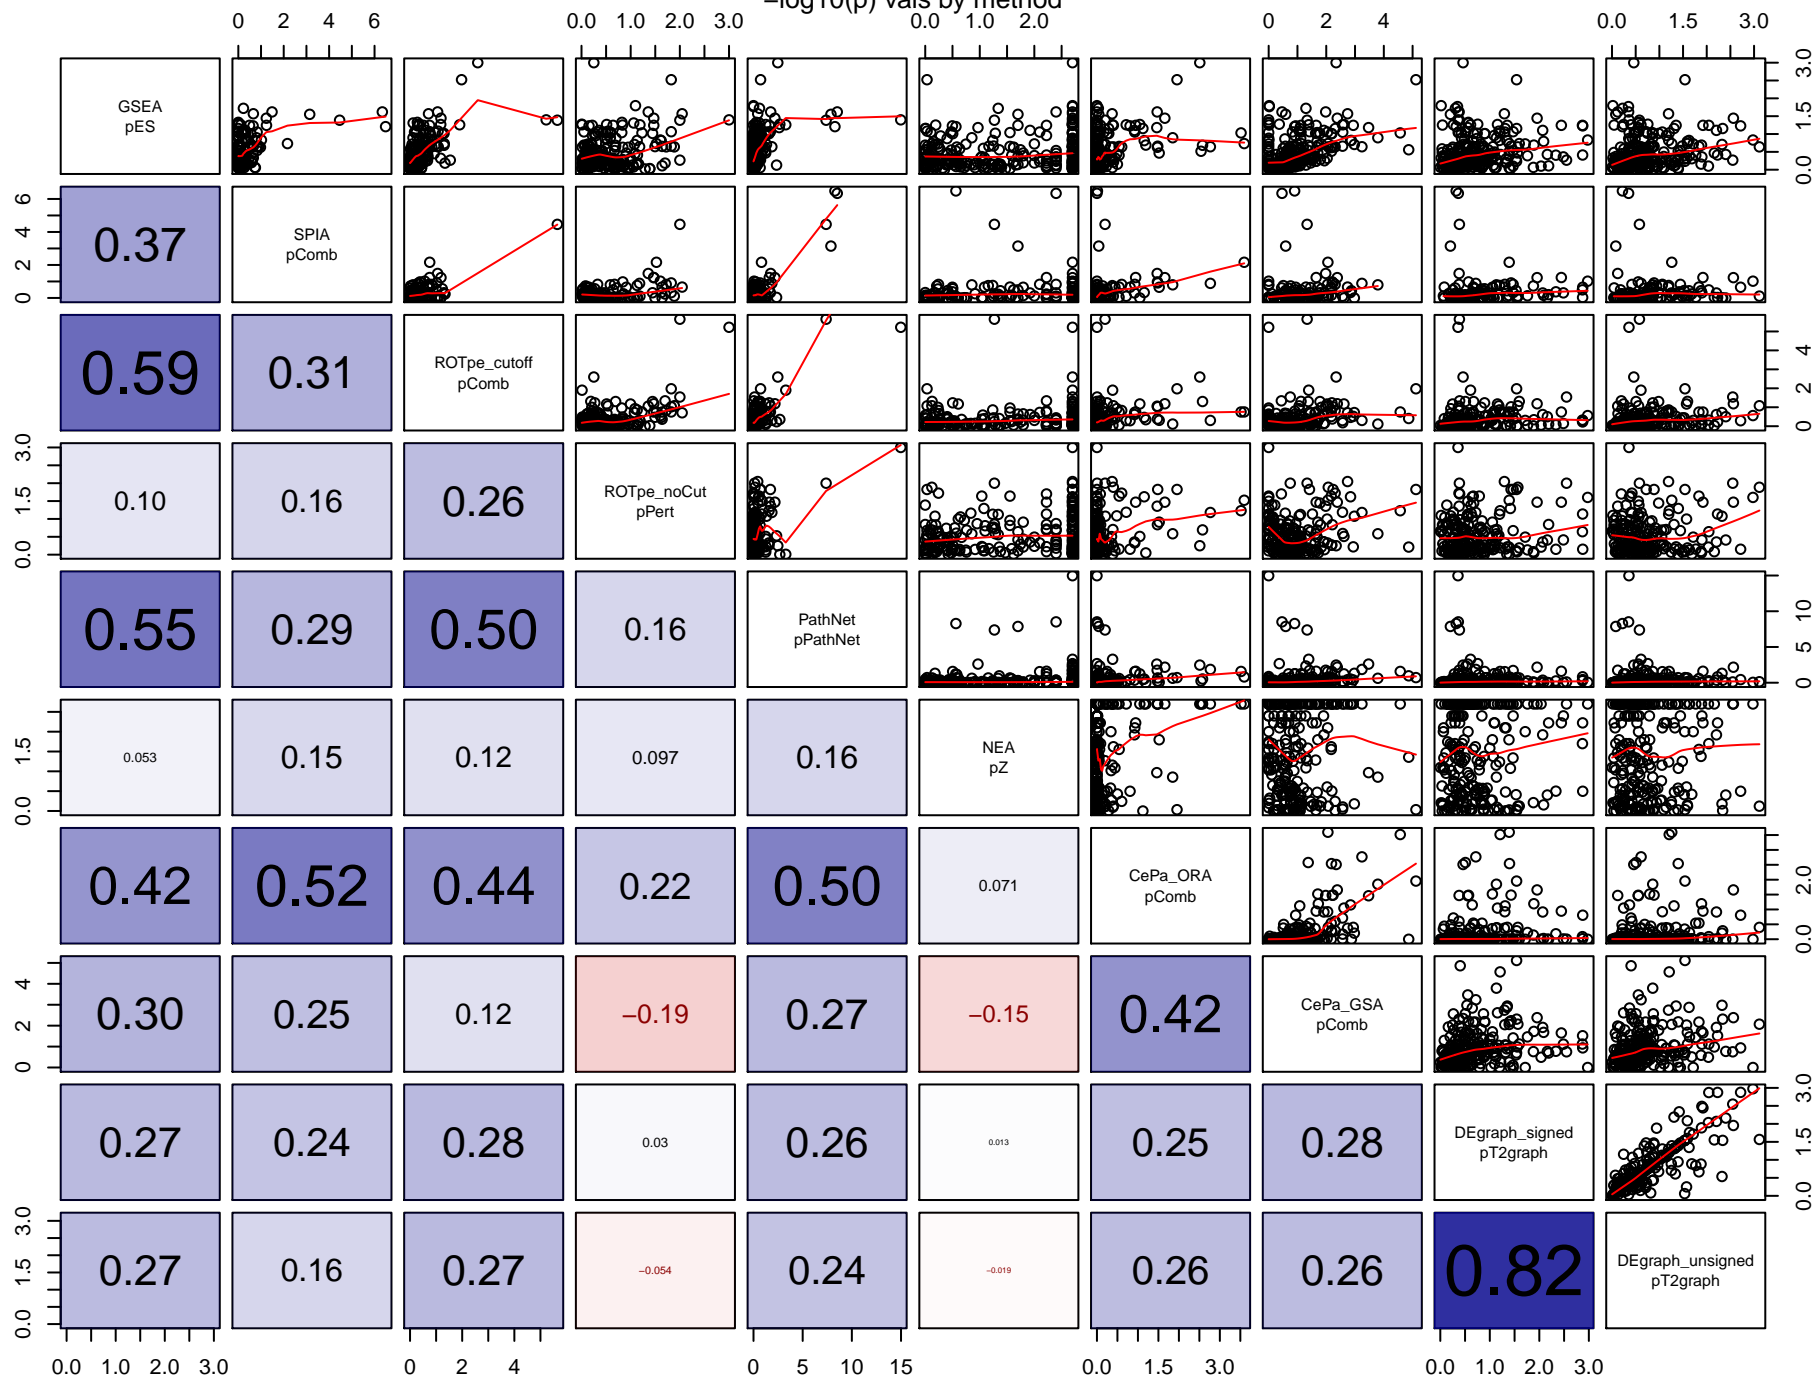

# GSE14764 data

-log10(p) vals by method

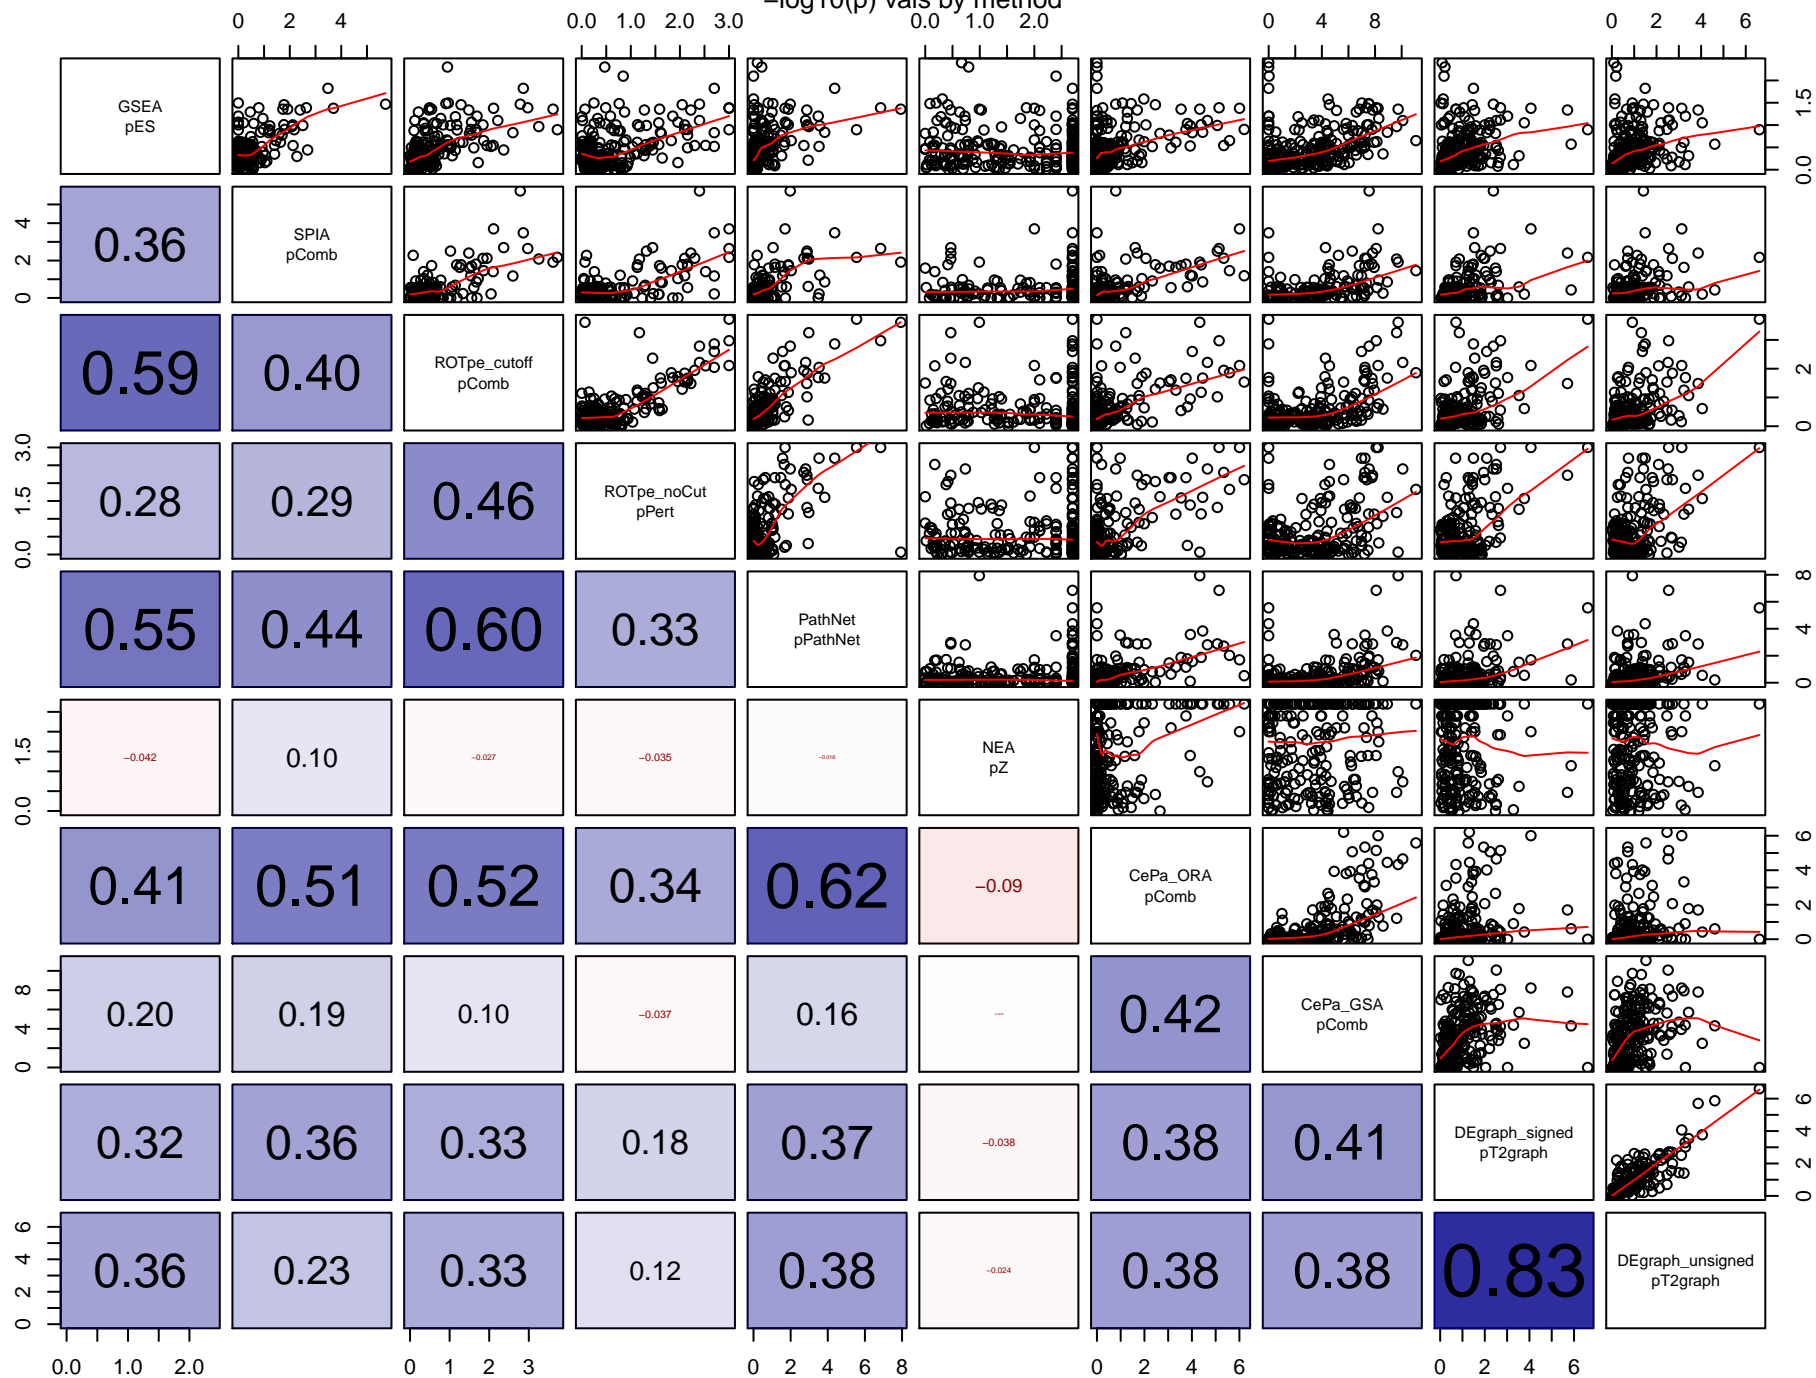

# GSE17260 data

-log10(p) vals by method

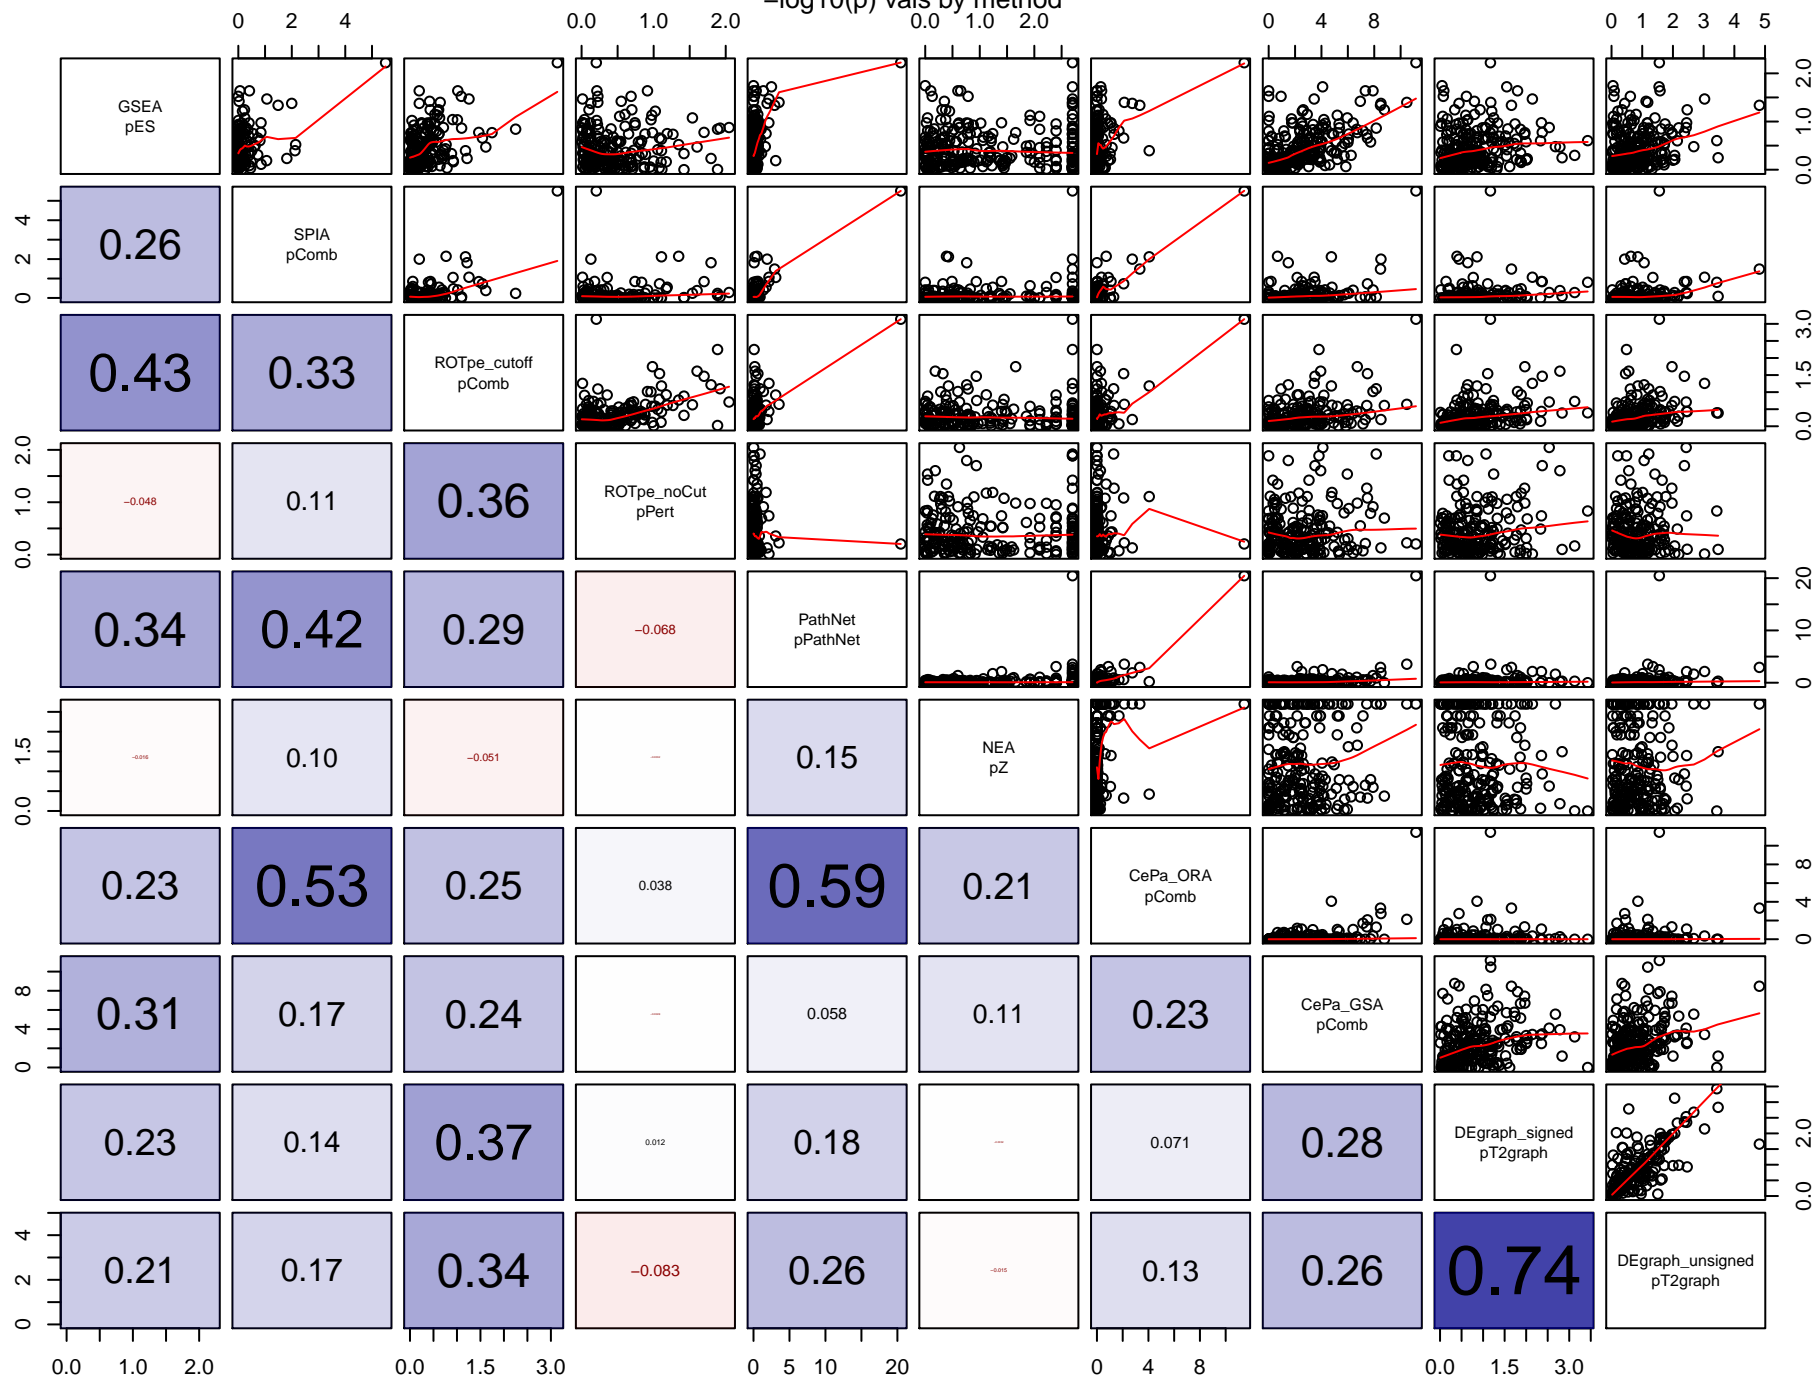

# GSE30161 data

-log10(p) vals by method

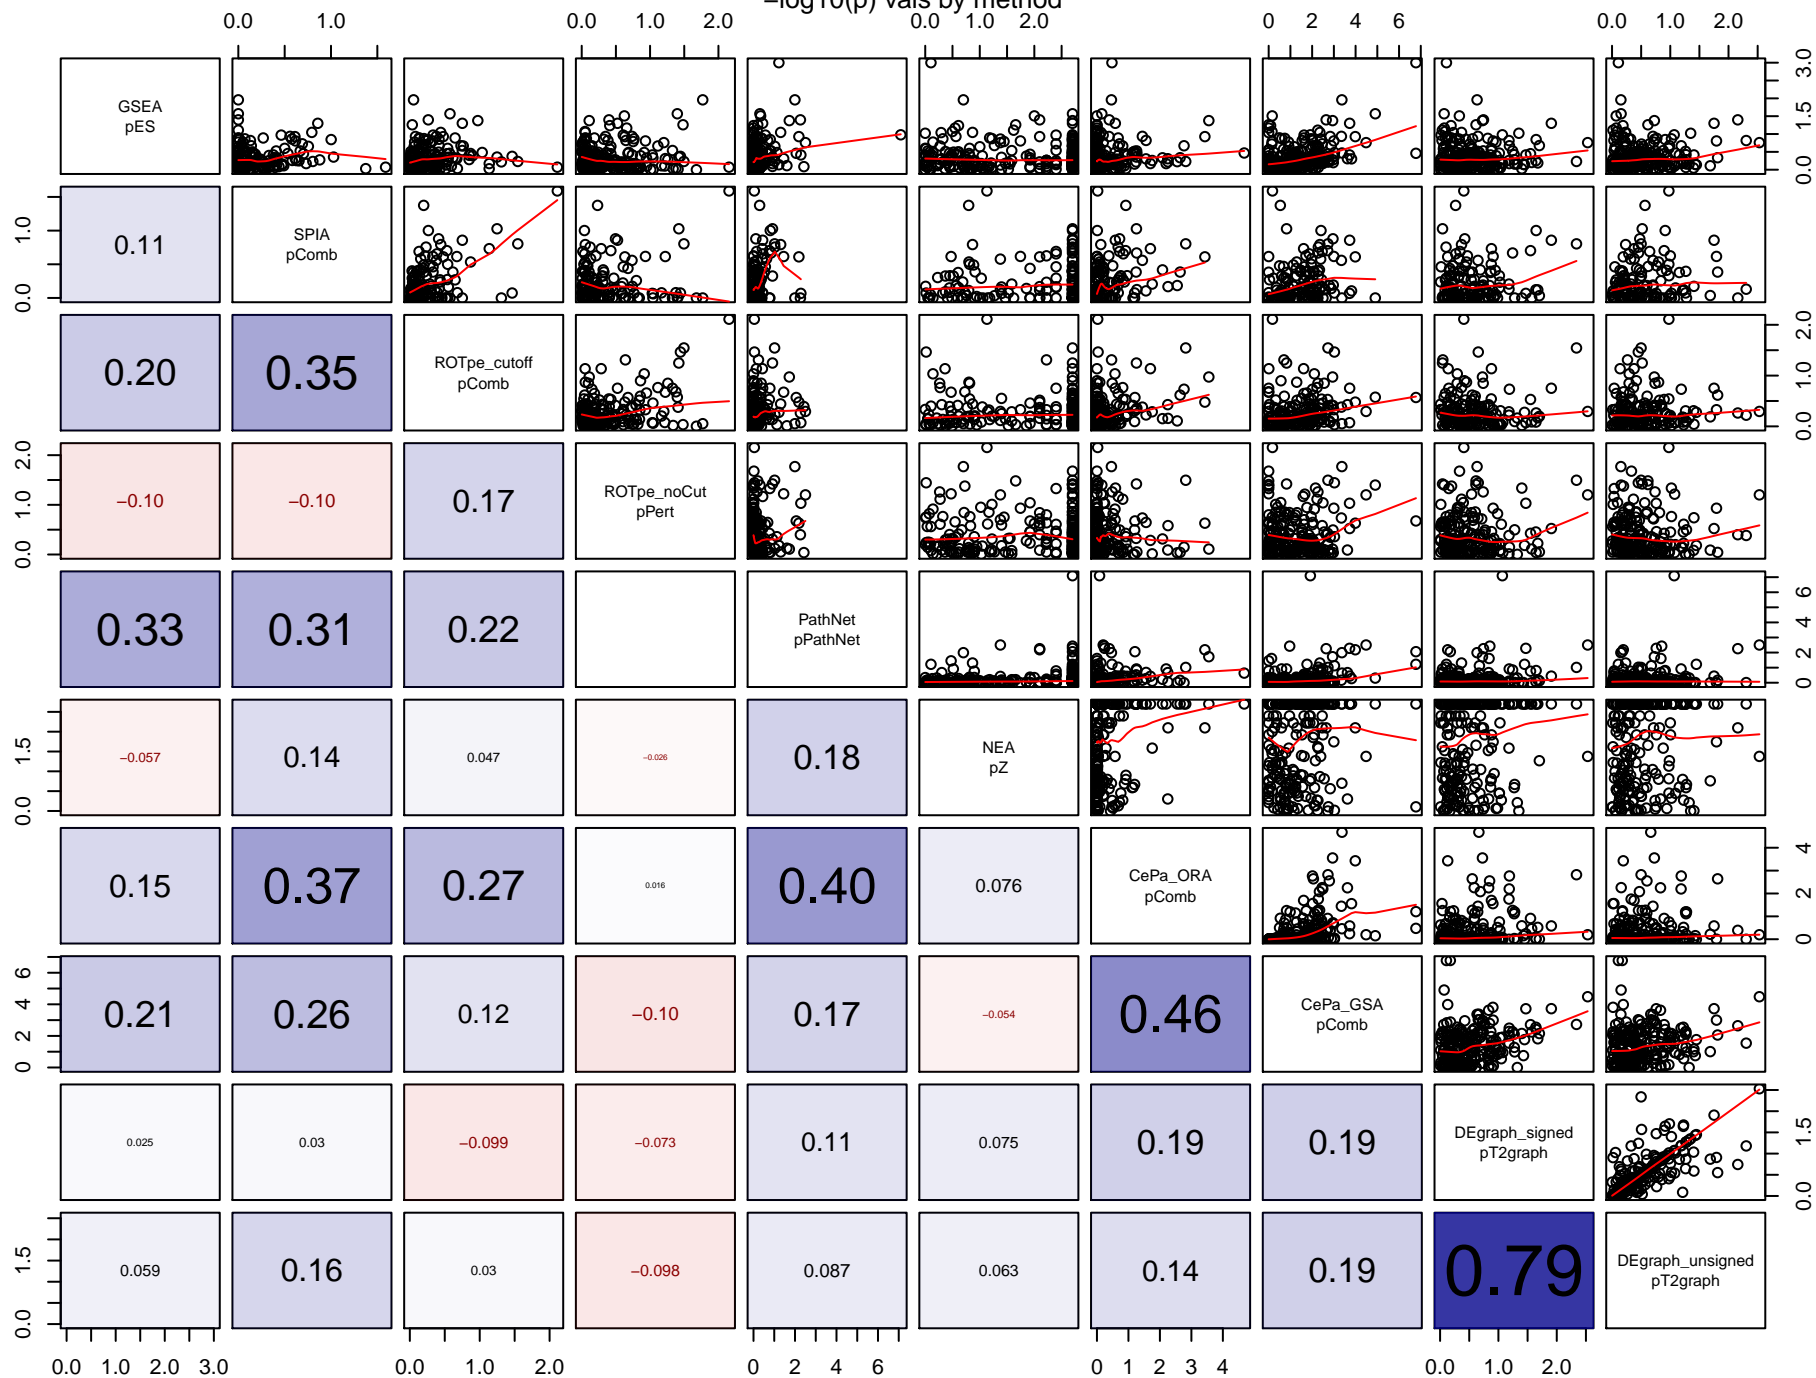

## GSE32062.GPL6480 data

-log10(p) vals by method

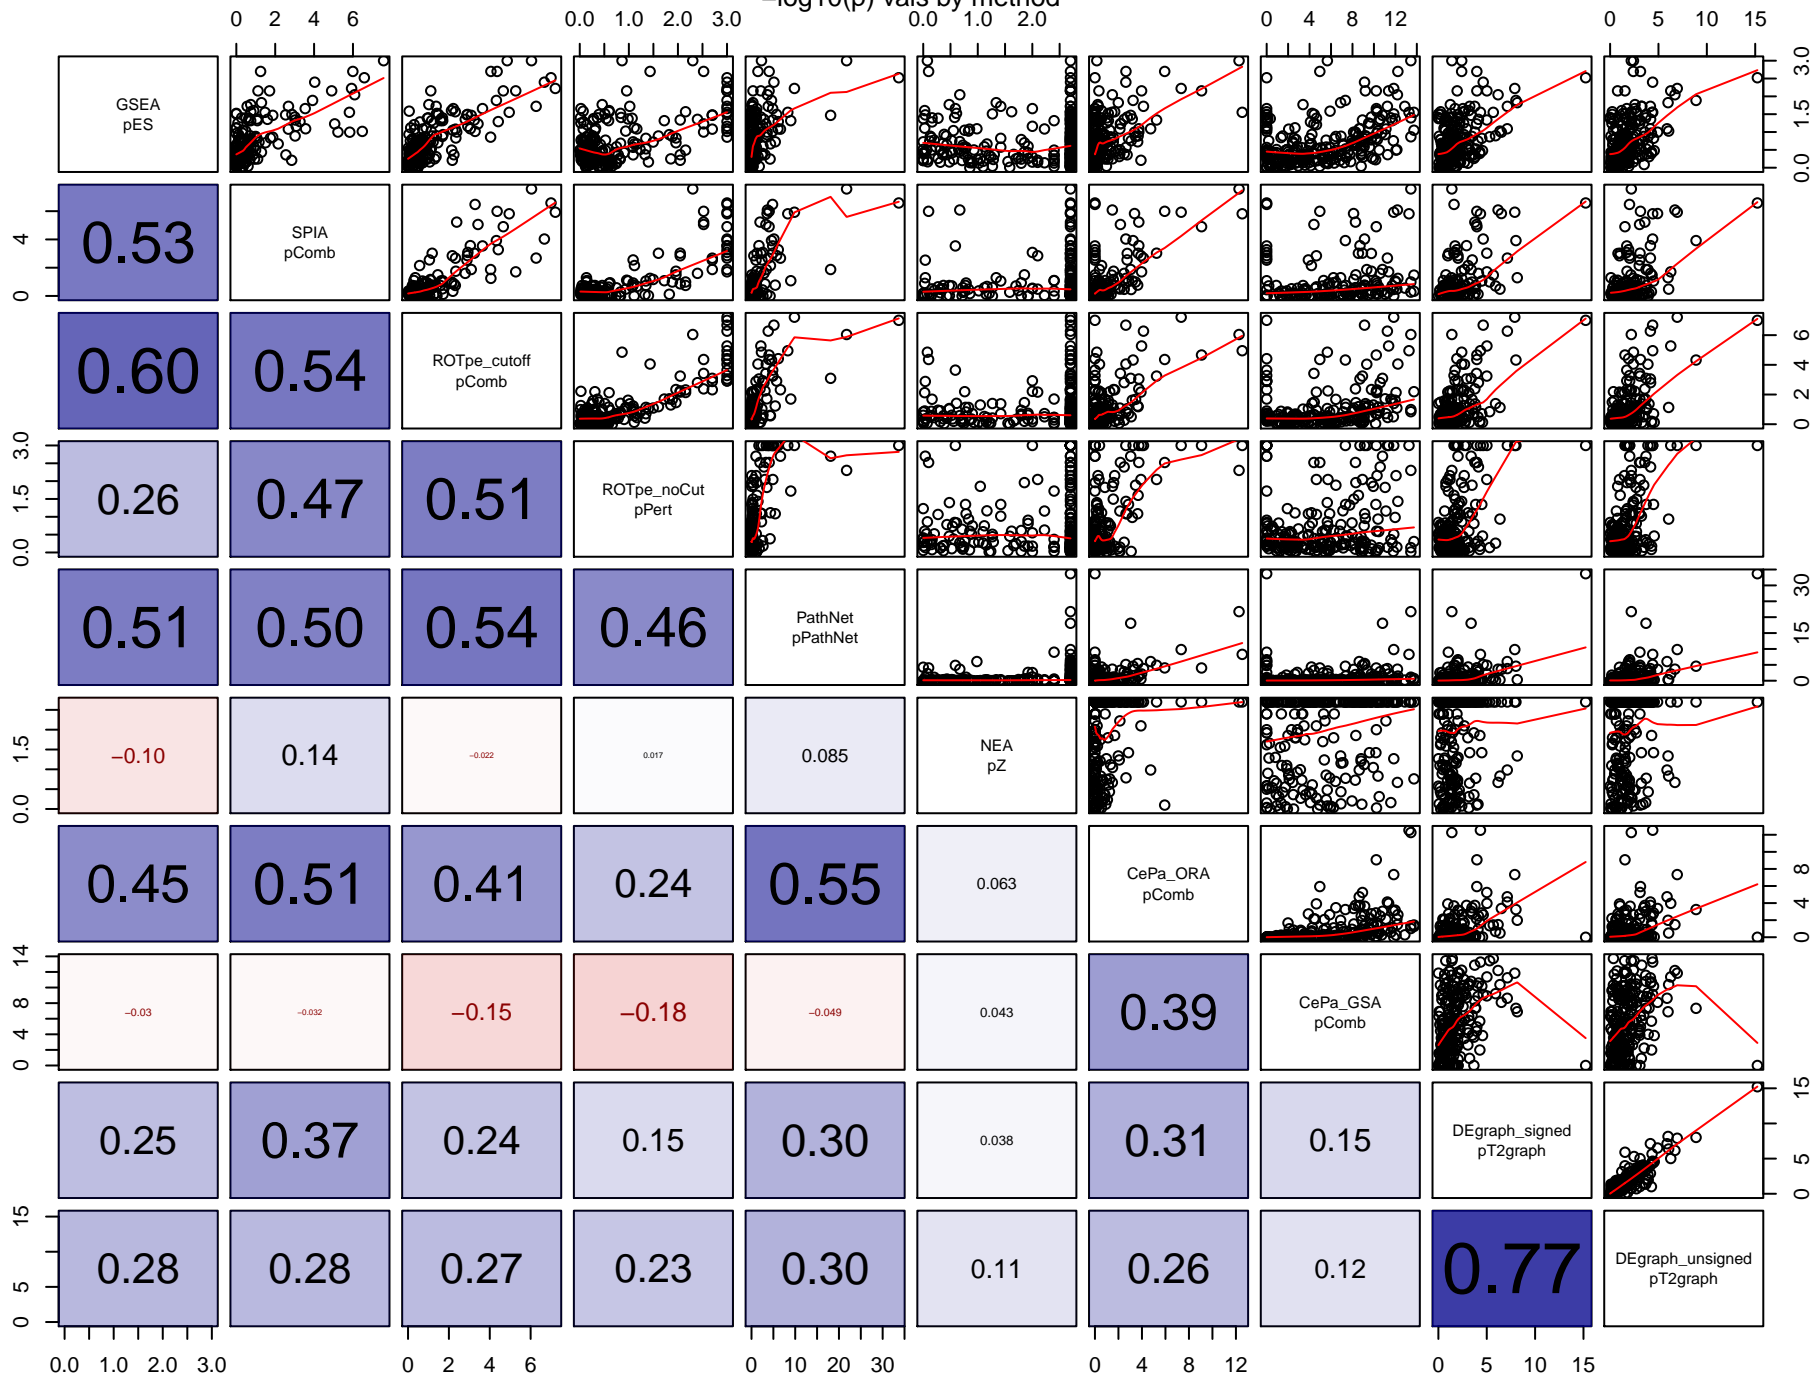

# GSE32063 data

-log10(p) vals by method

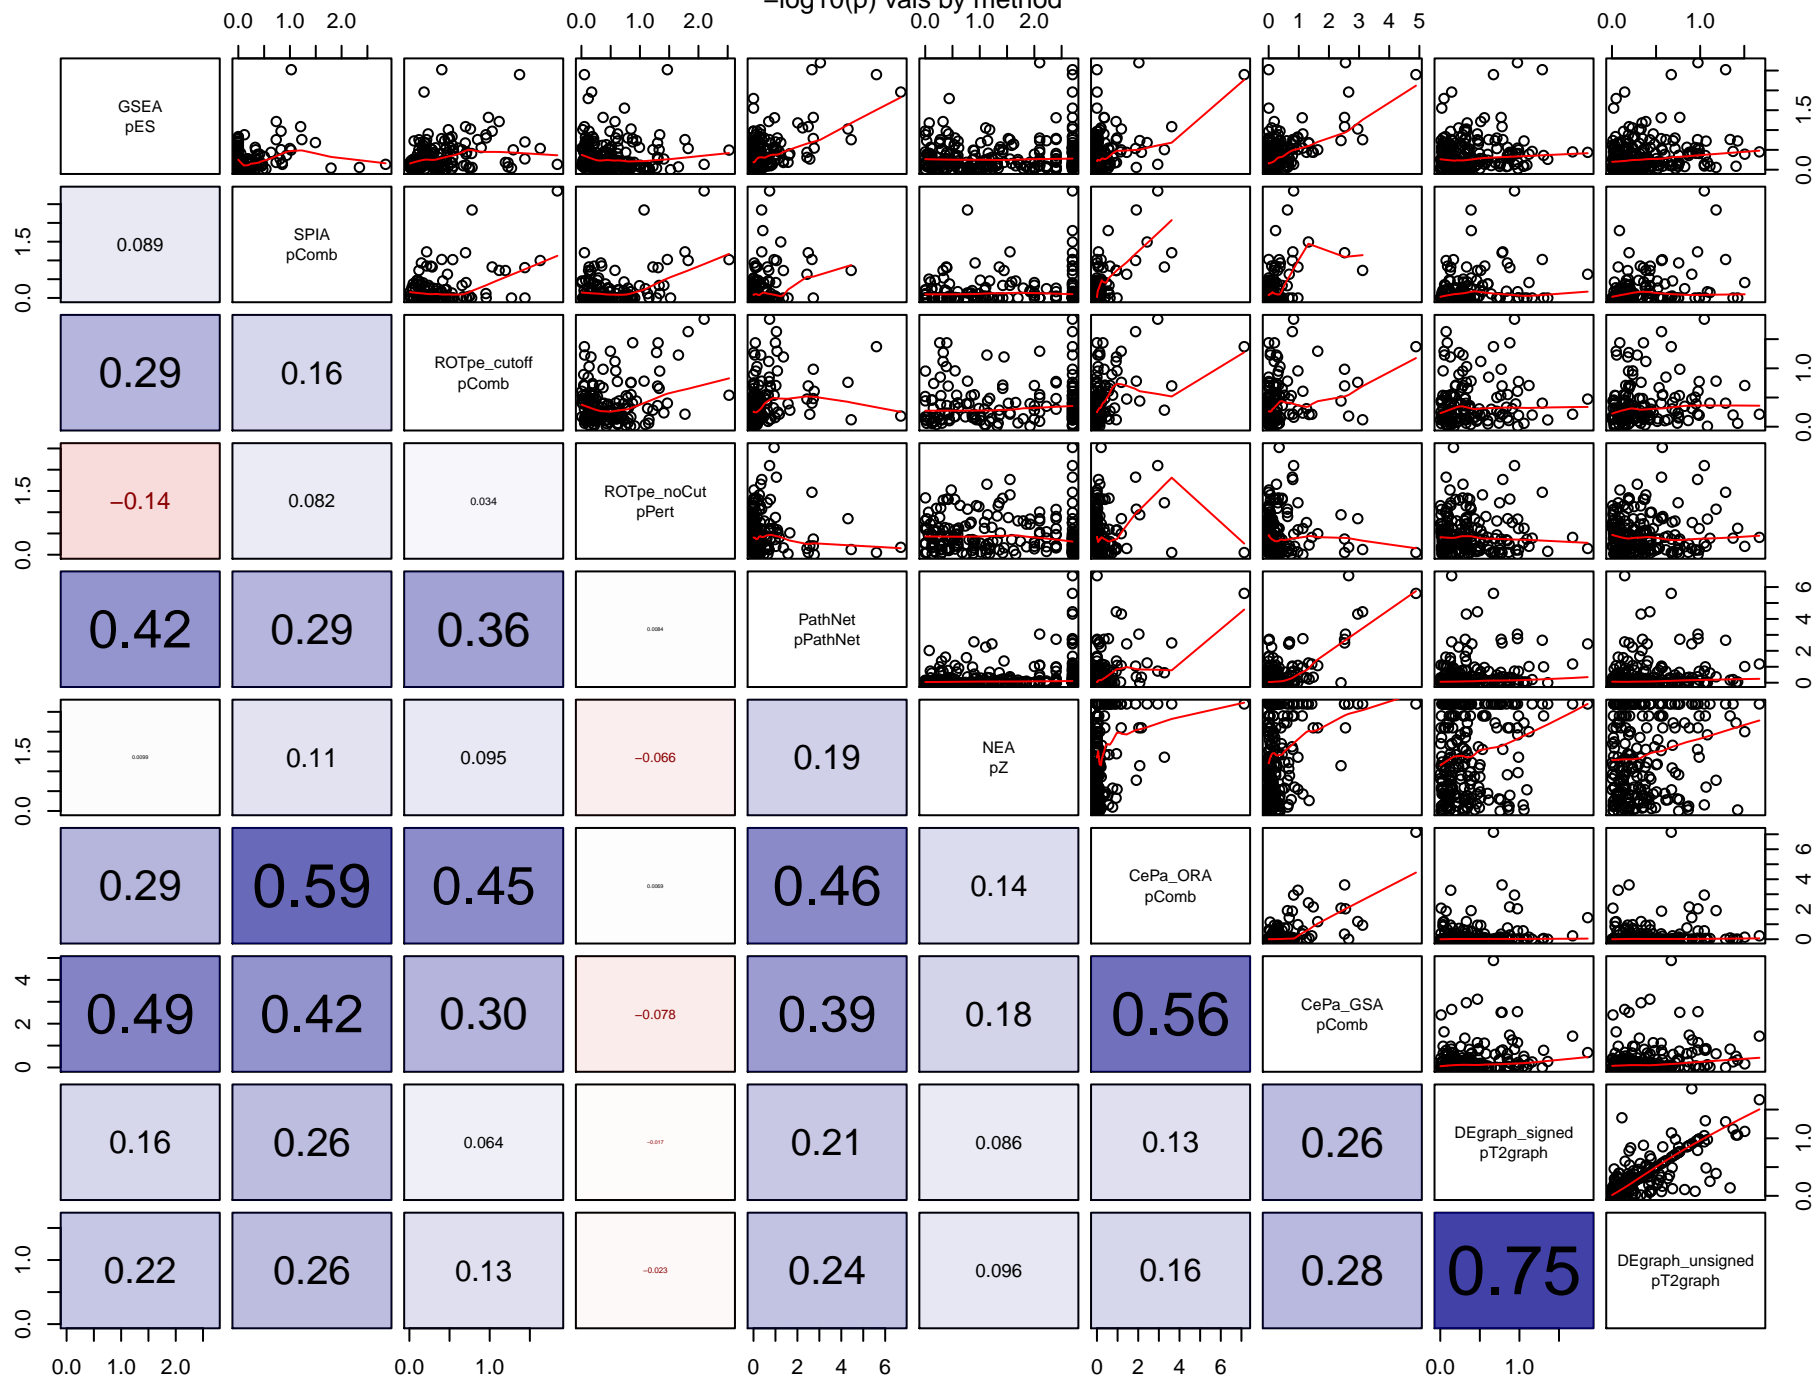



# GSE9891 data

-log10(p) vals by method

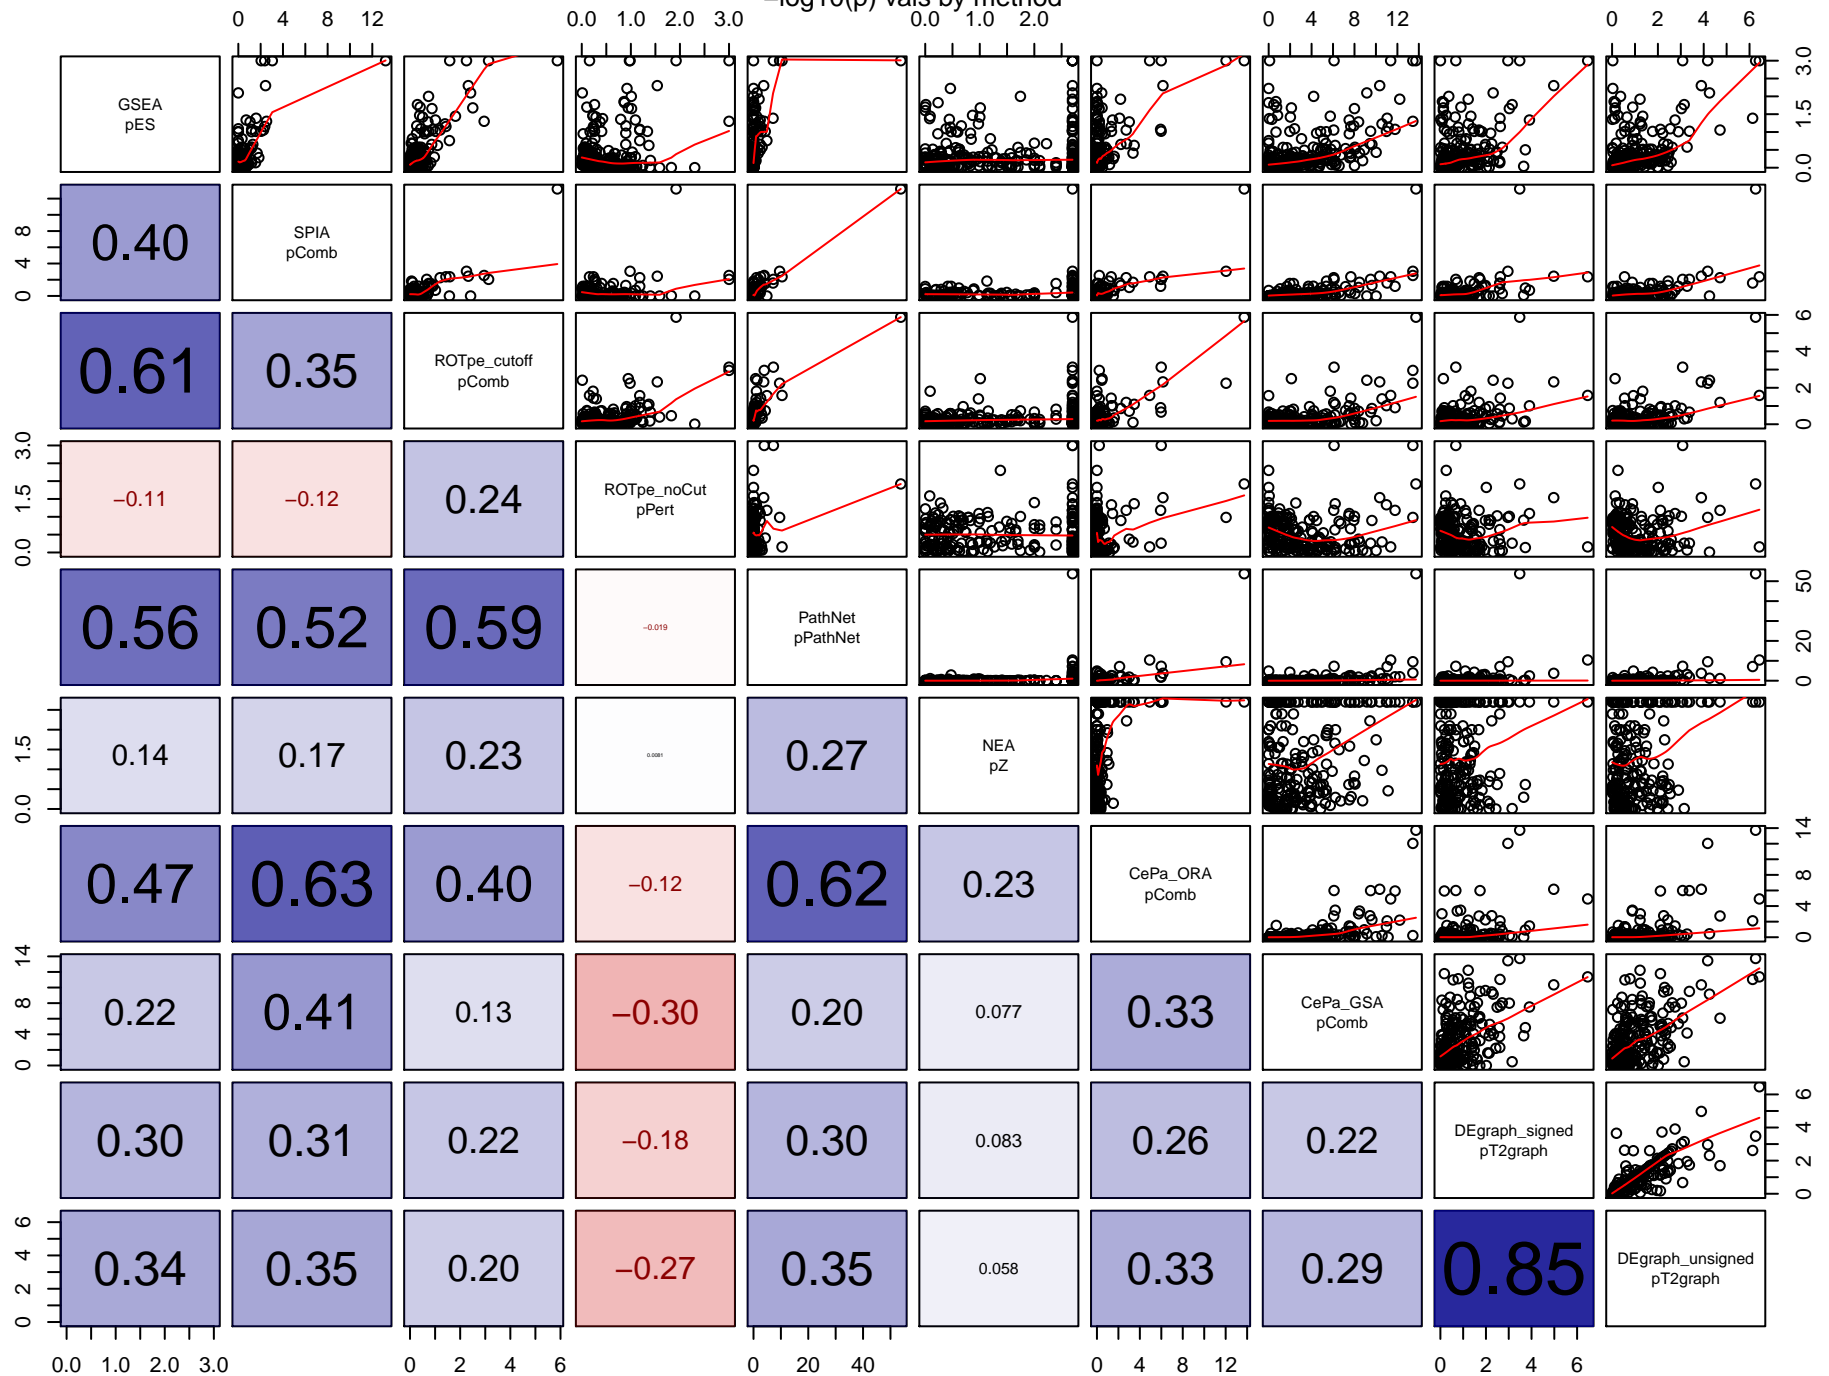

# PMID17290060 data

-log10(p) vals by method

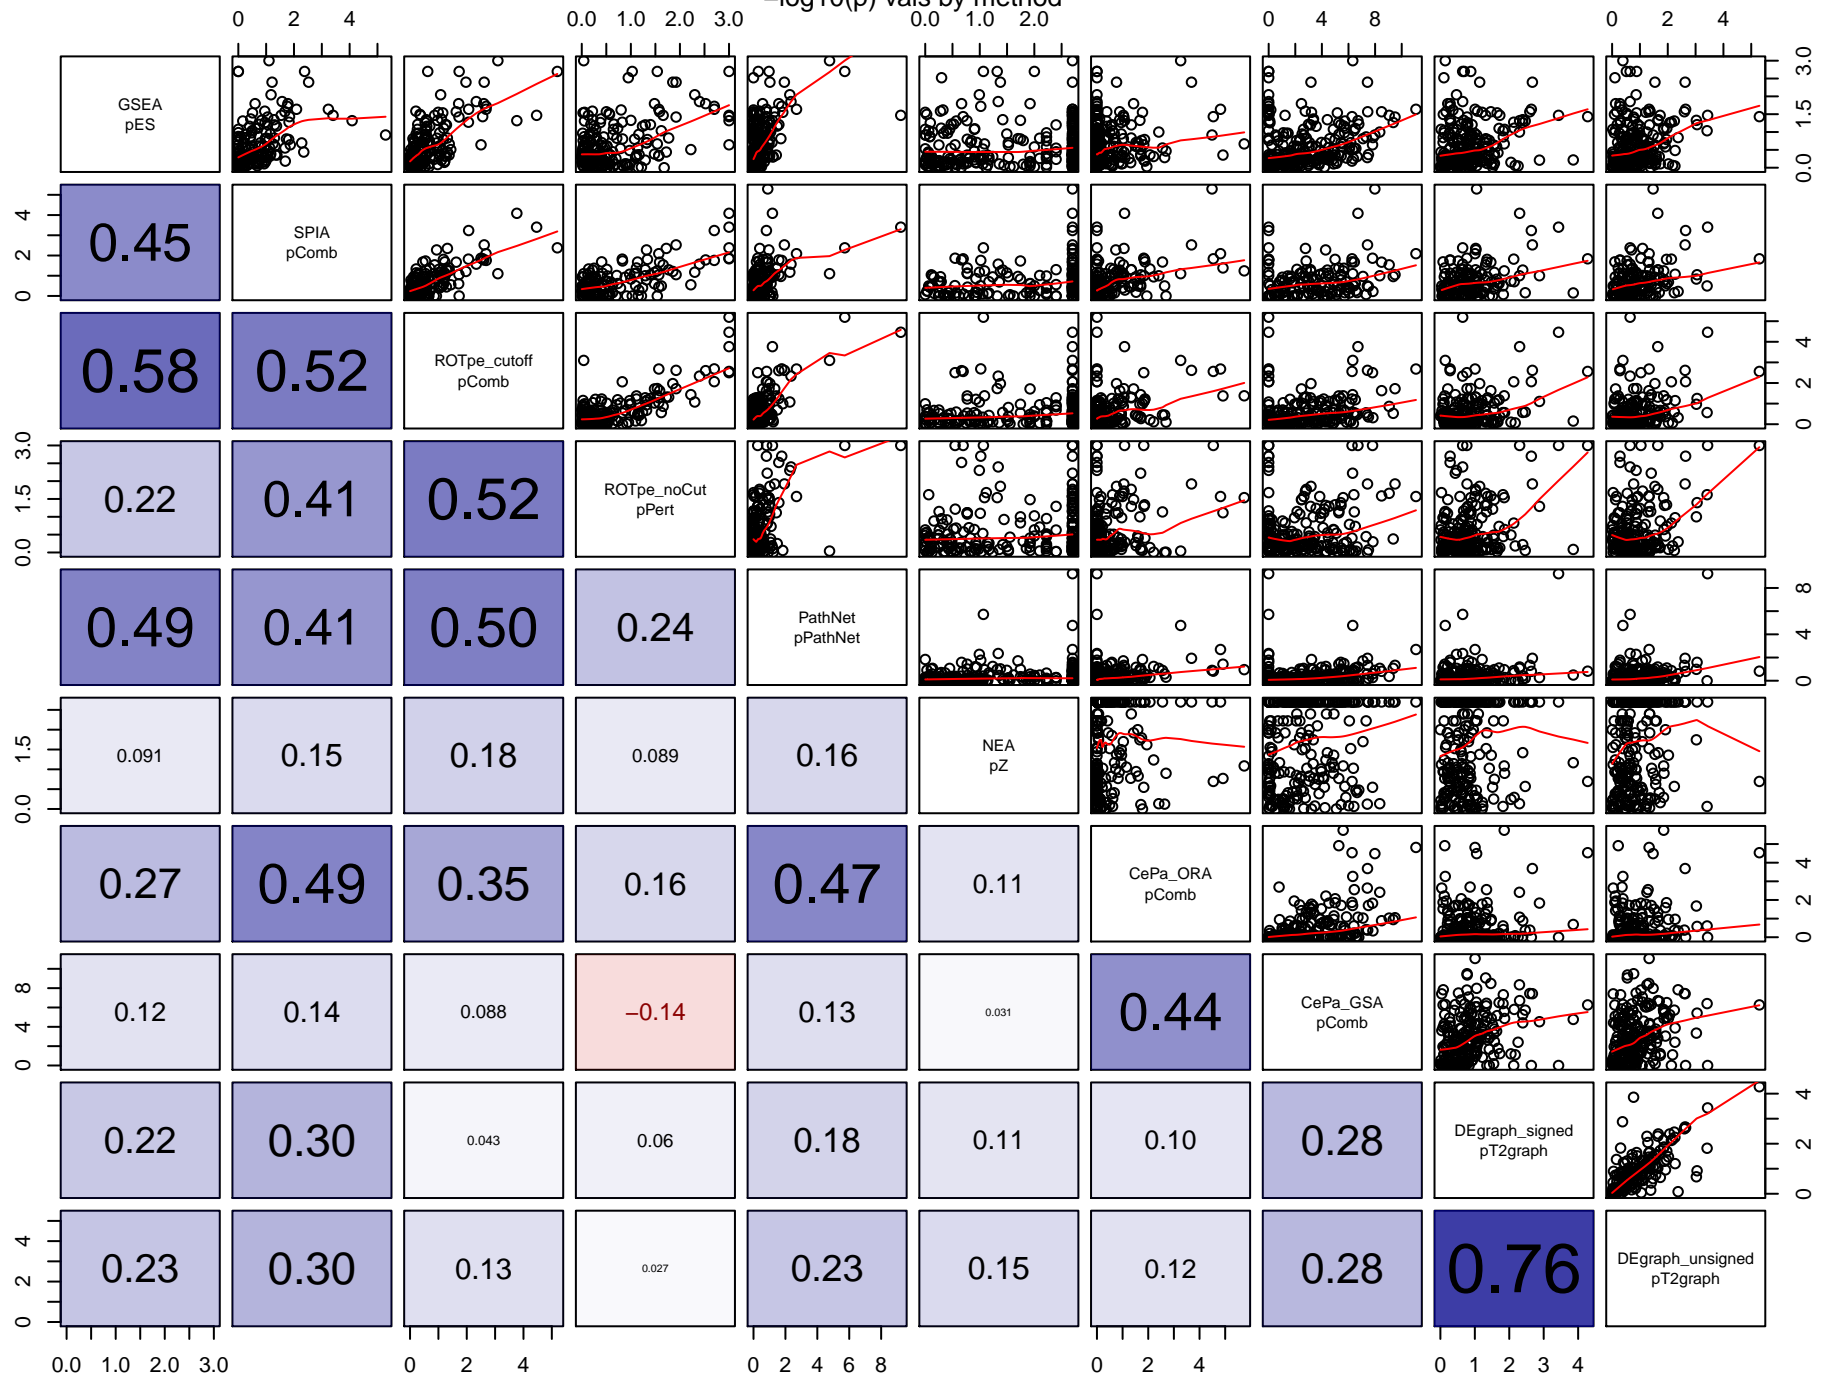



# PMID19318476 data

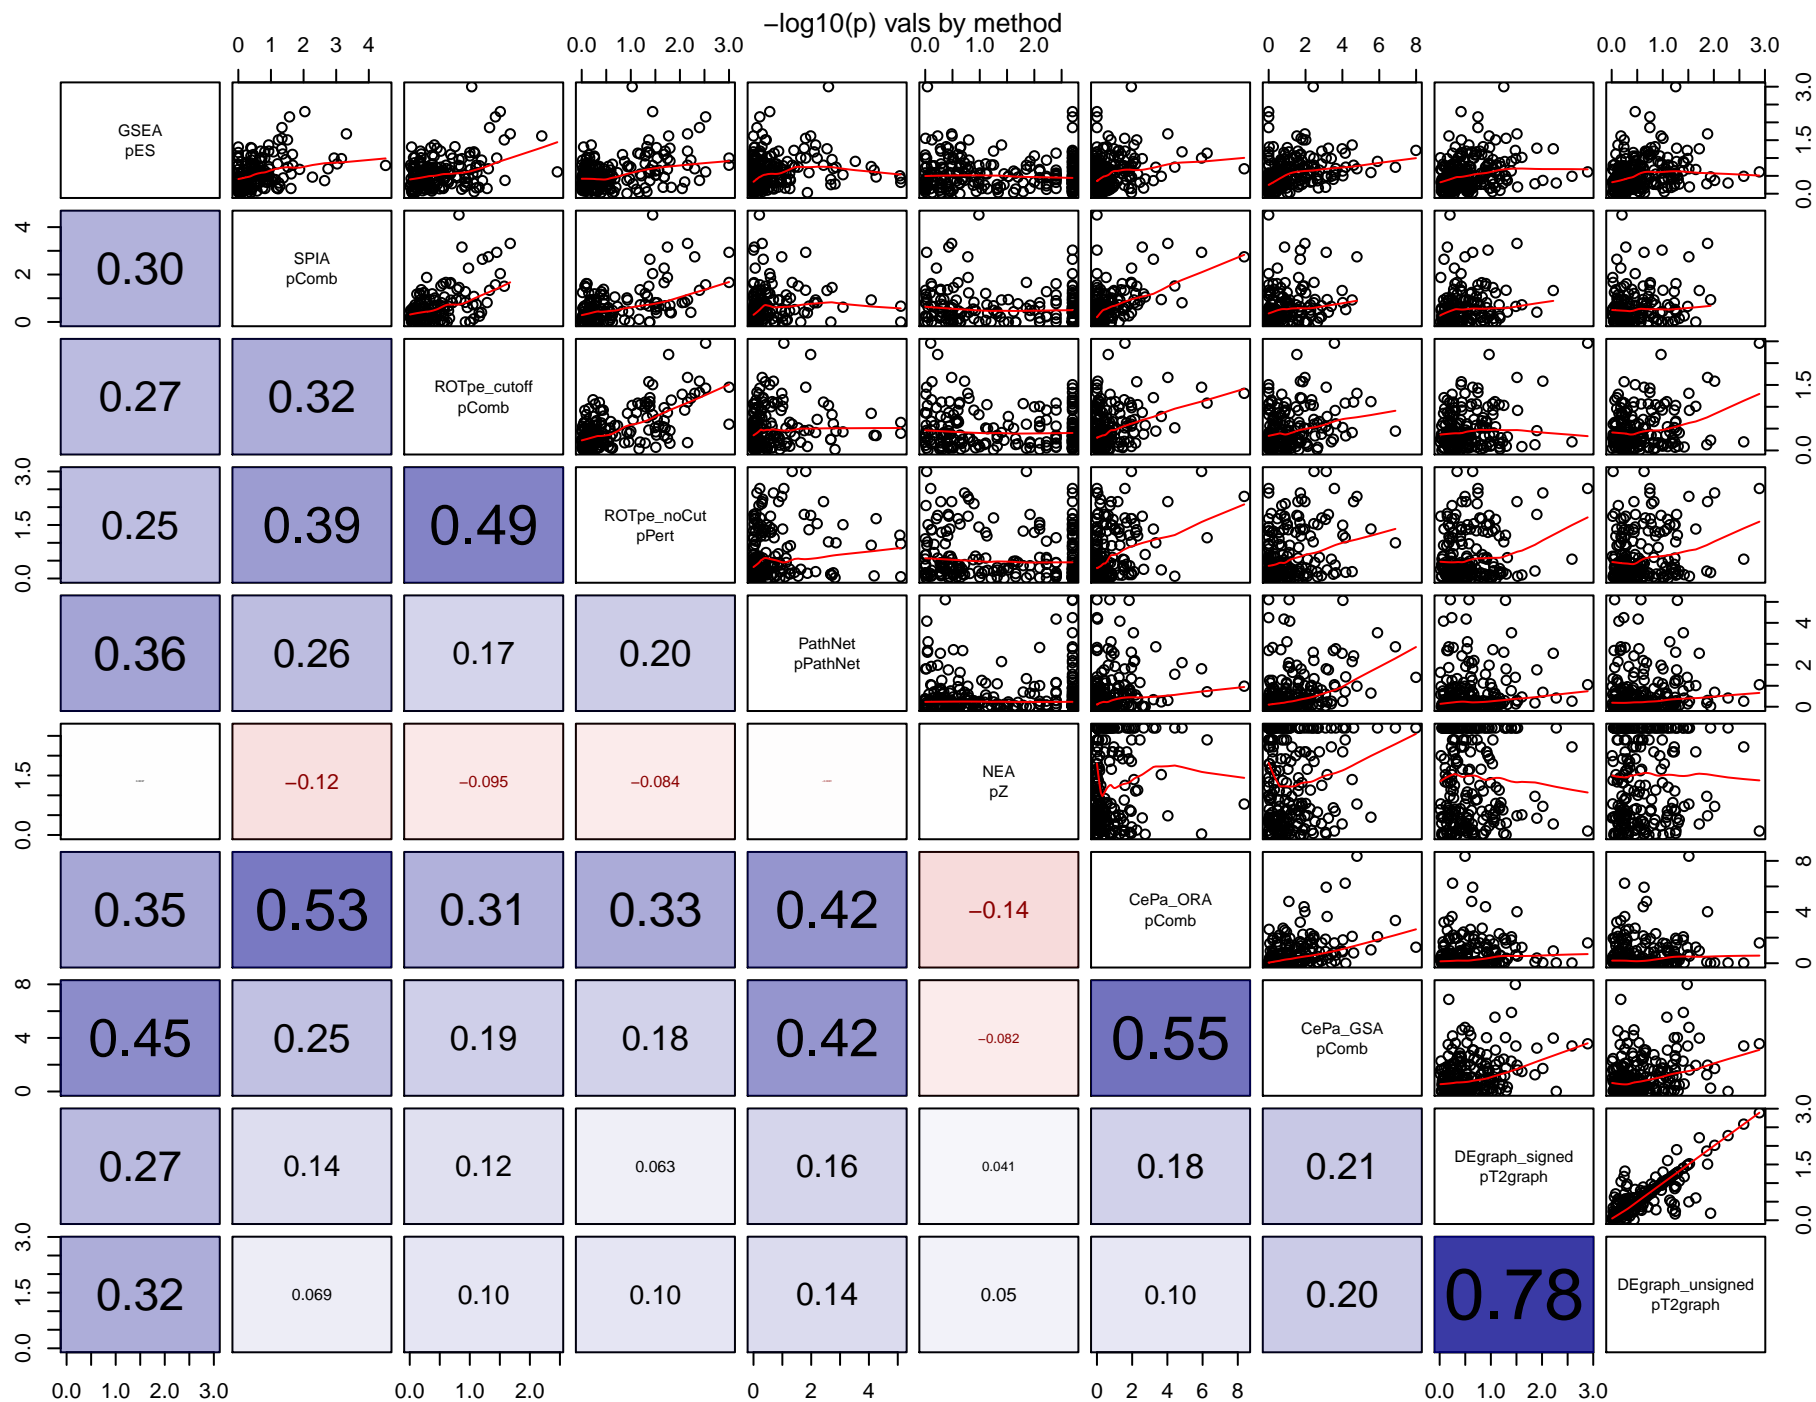

# TCGA data

-log10(p) vals by method

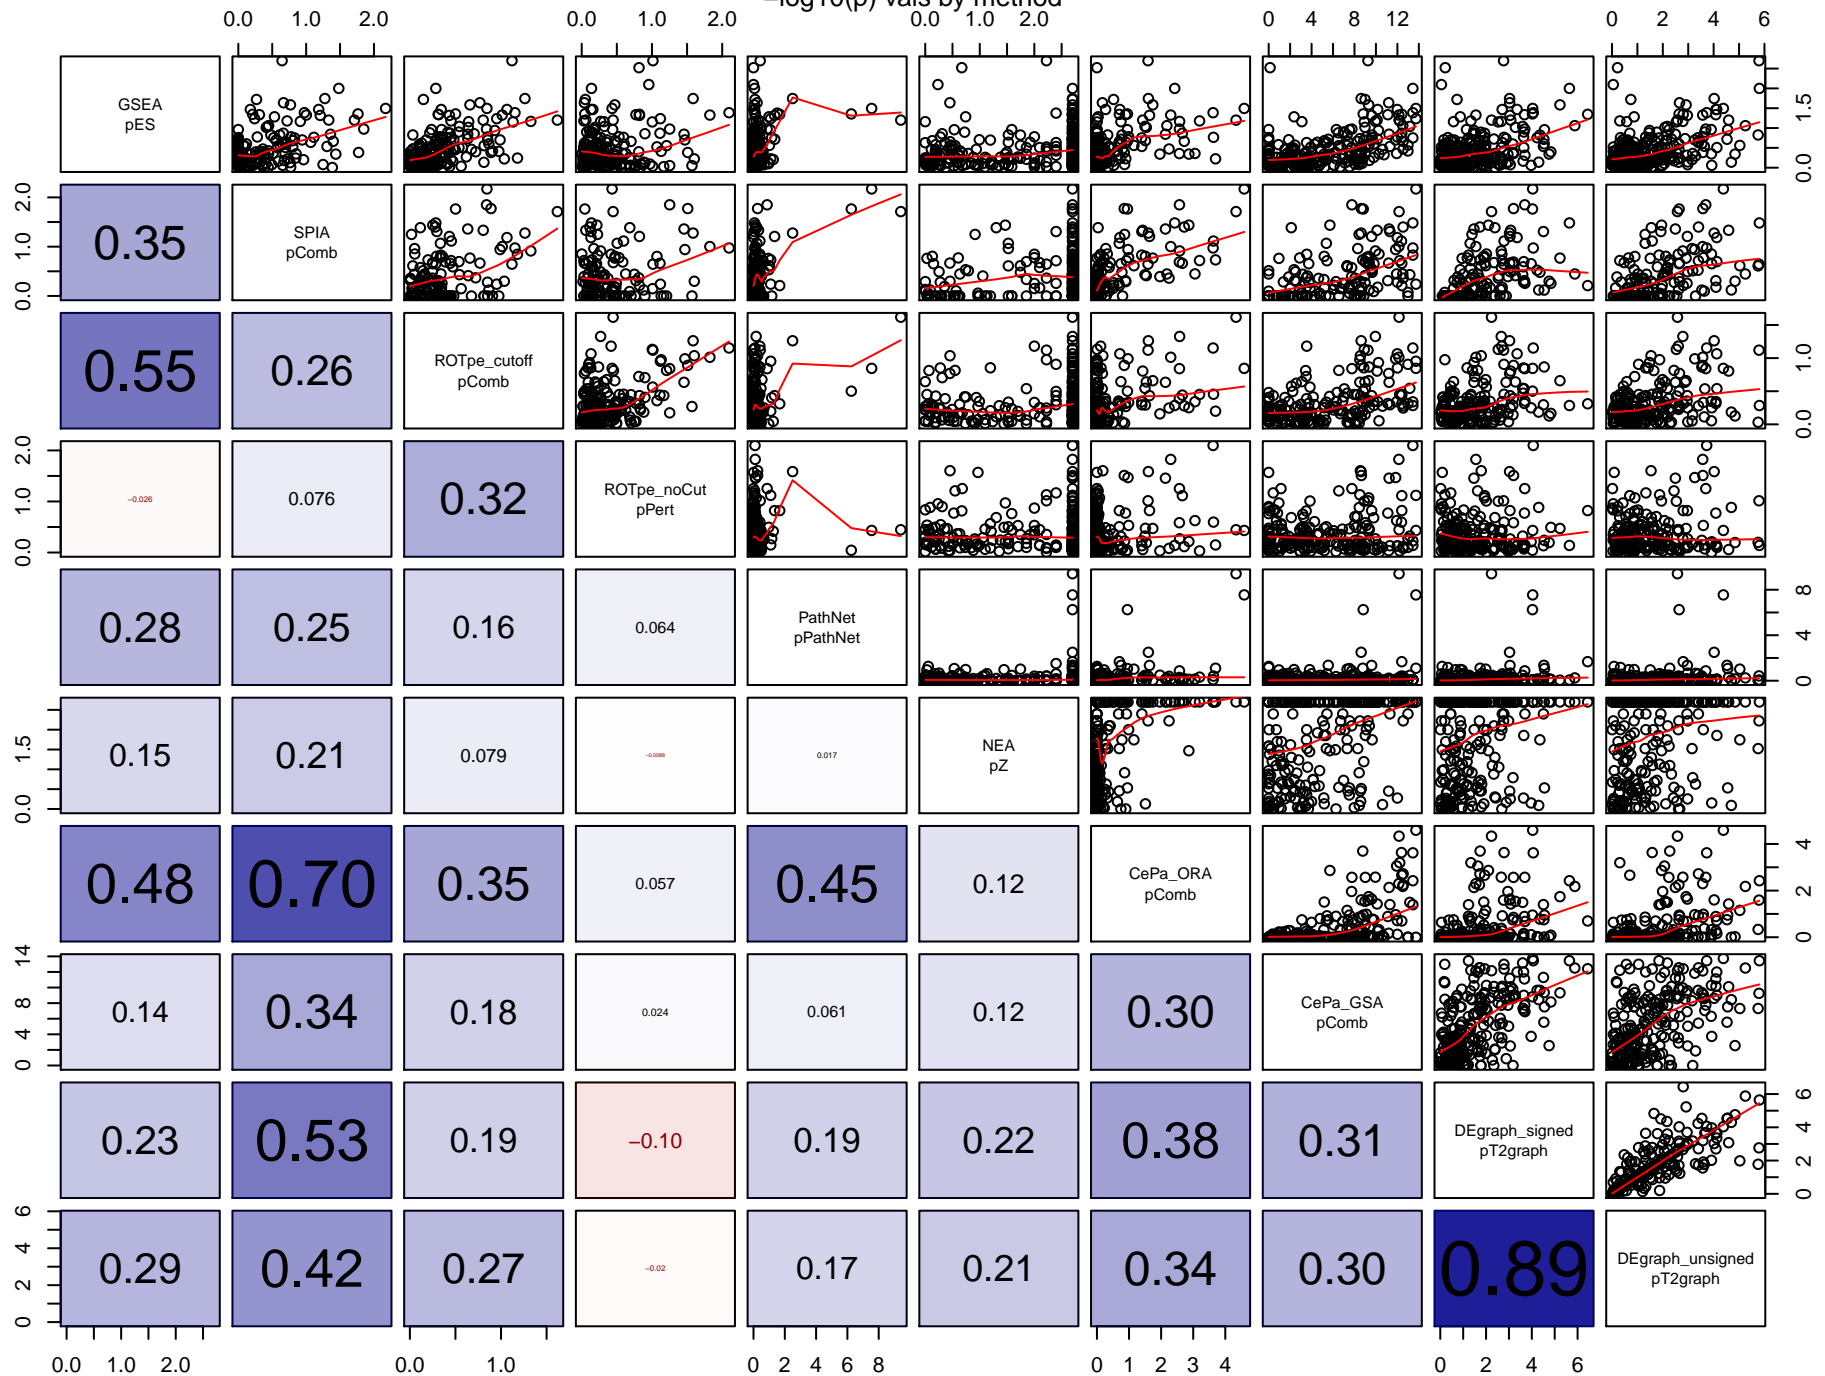

Supplement: Supplementary file 1 [file supp.xMethodPairs.pdf]
