# Supplementary material for: Network Methods for Pathway Analysis of Genomic Data
Source: arXiv:1411.1993 source file (2014-11-07)

# gene-level analysis

$-\log_{10}(p)$  vals by study

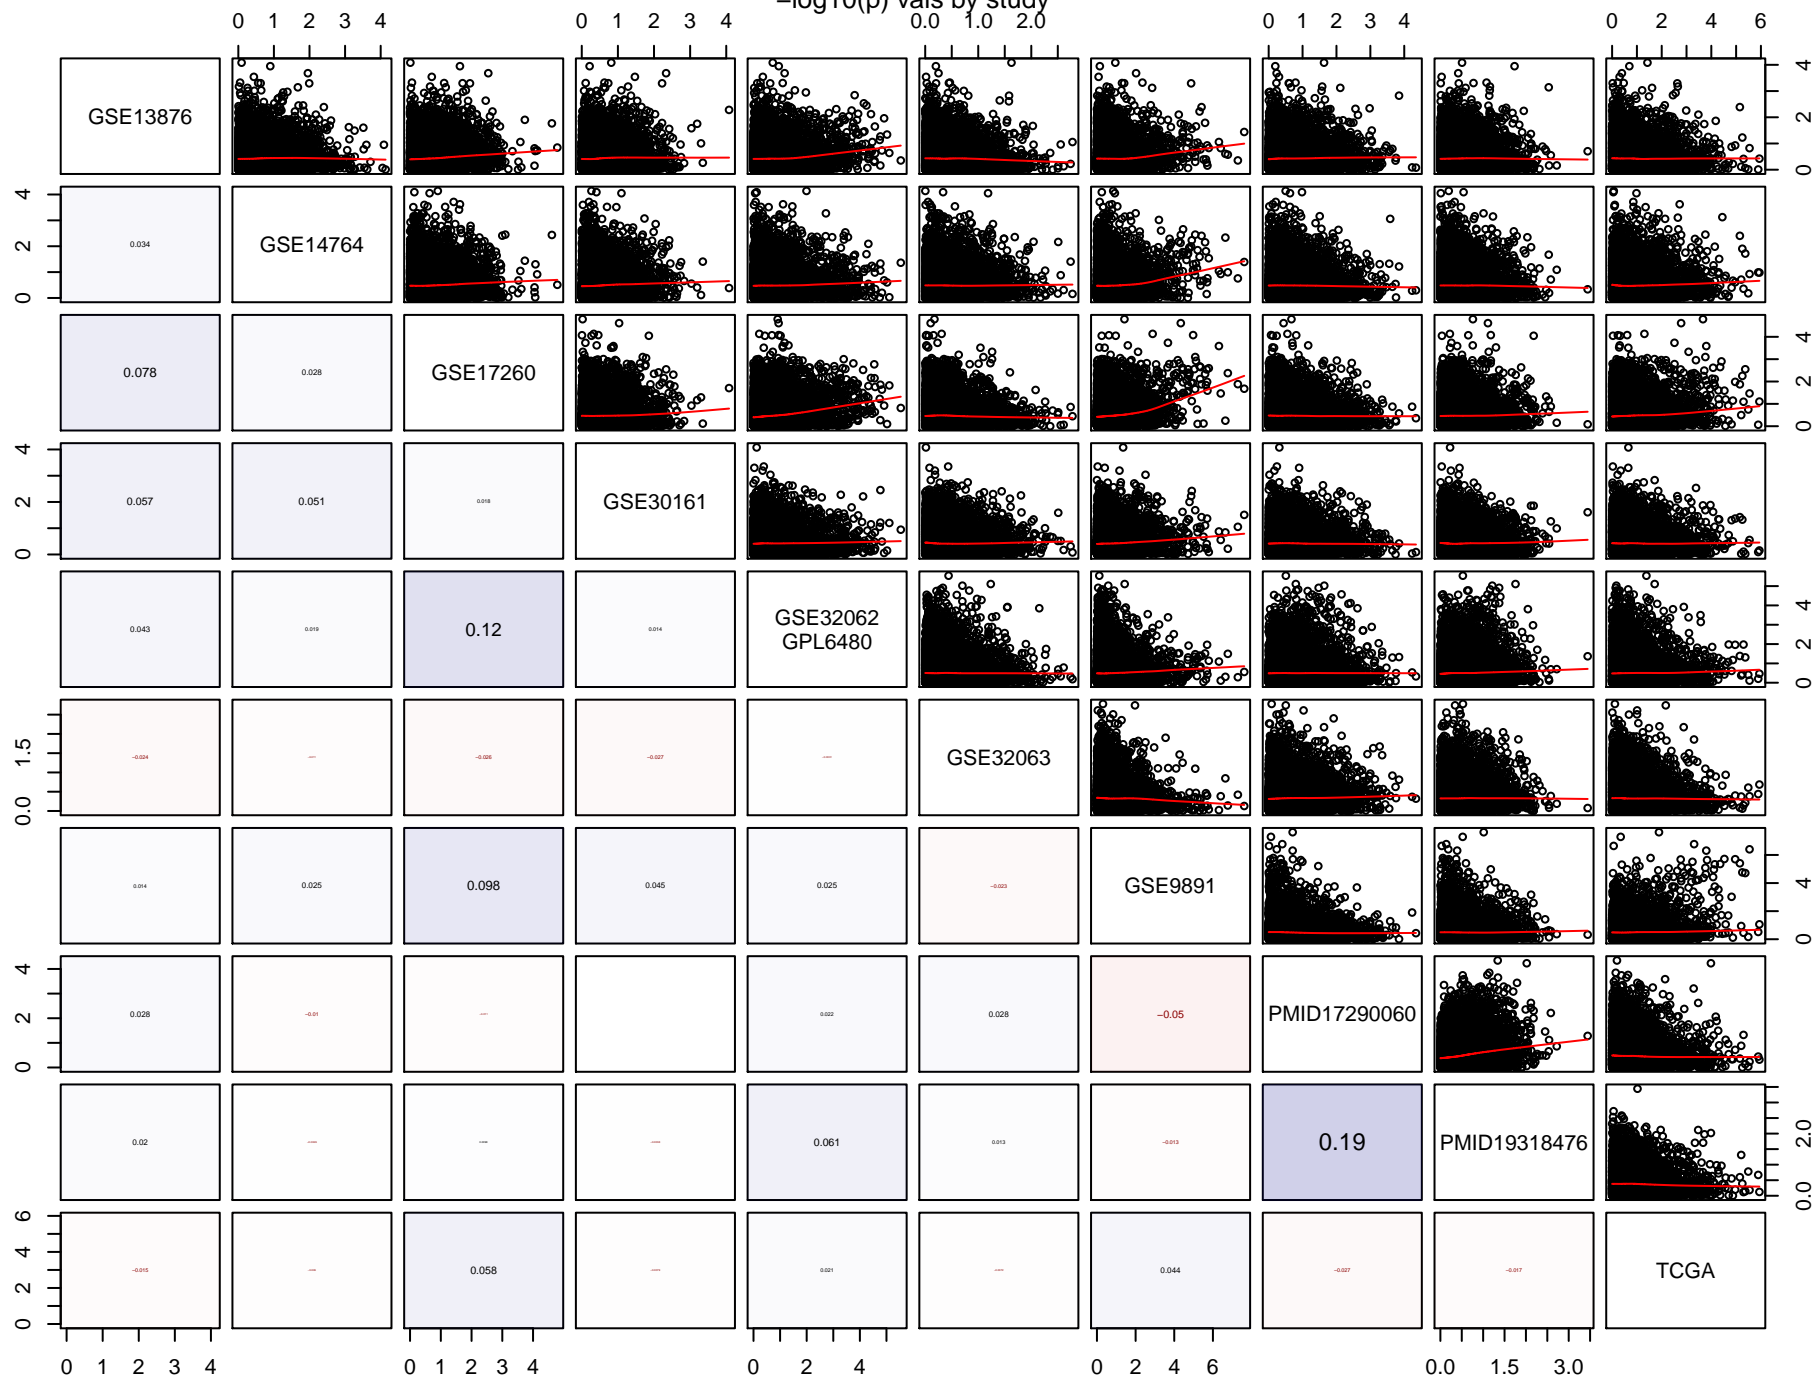

# GSEA.pES analysis

-log10(p) vals by study

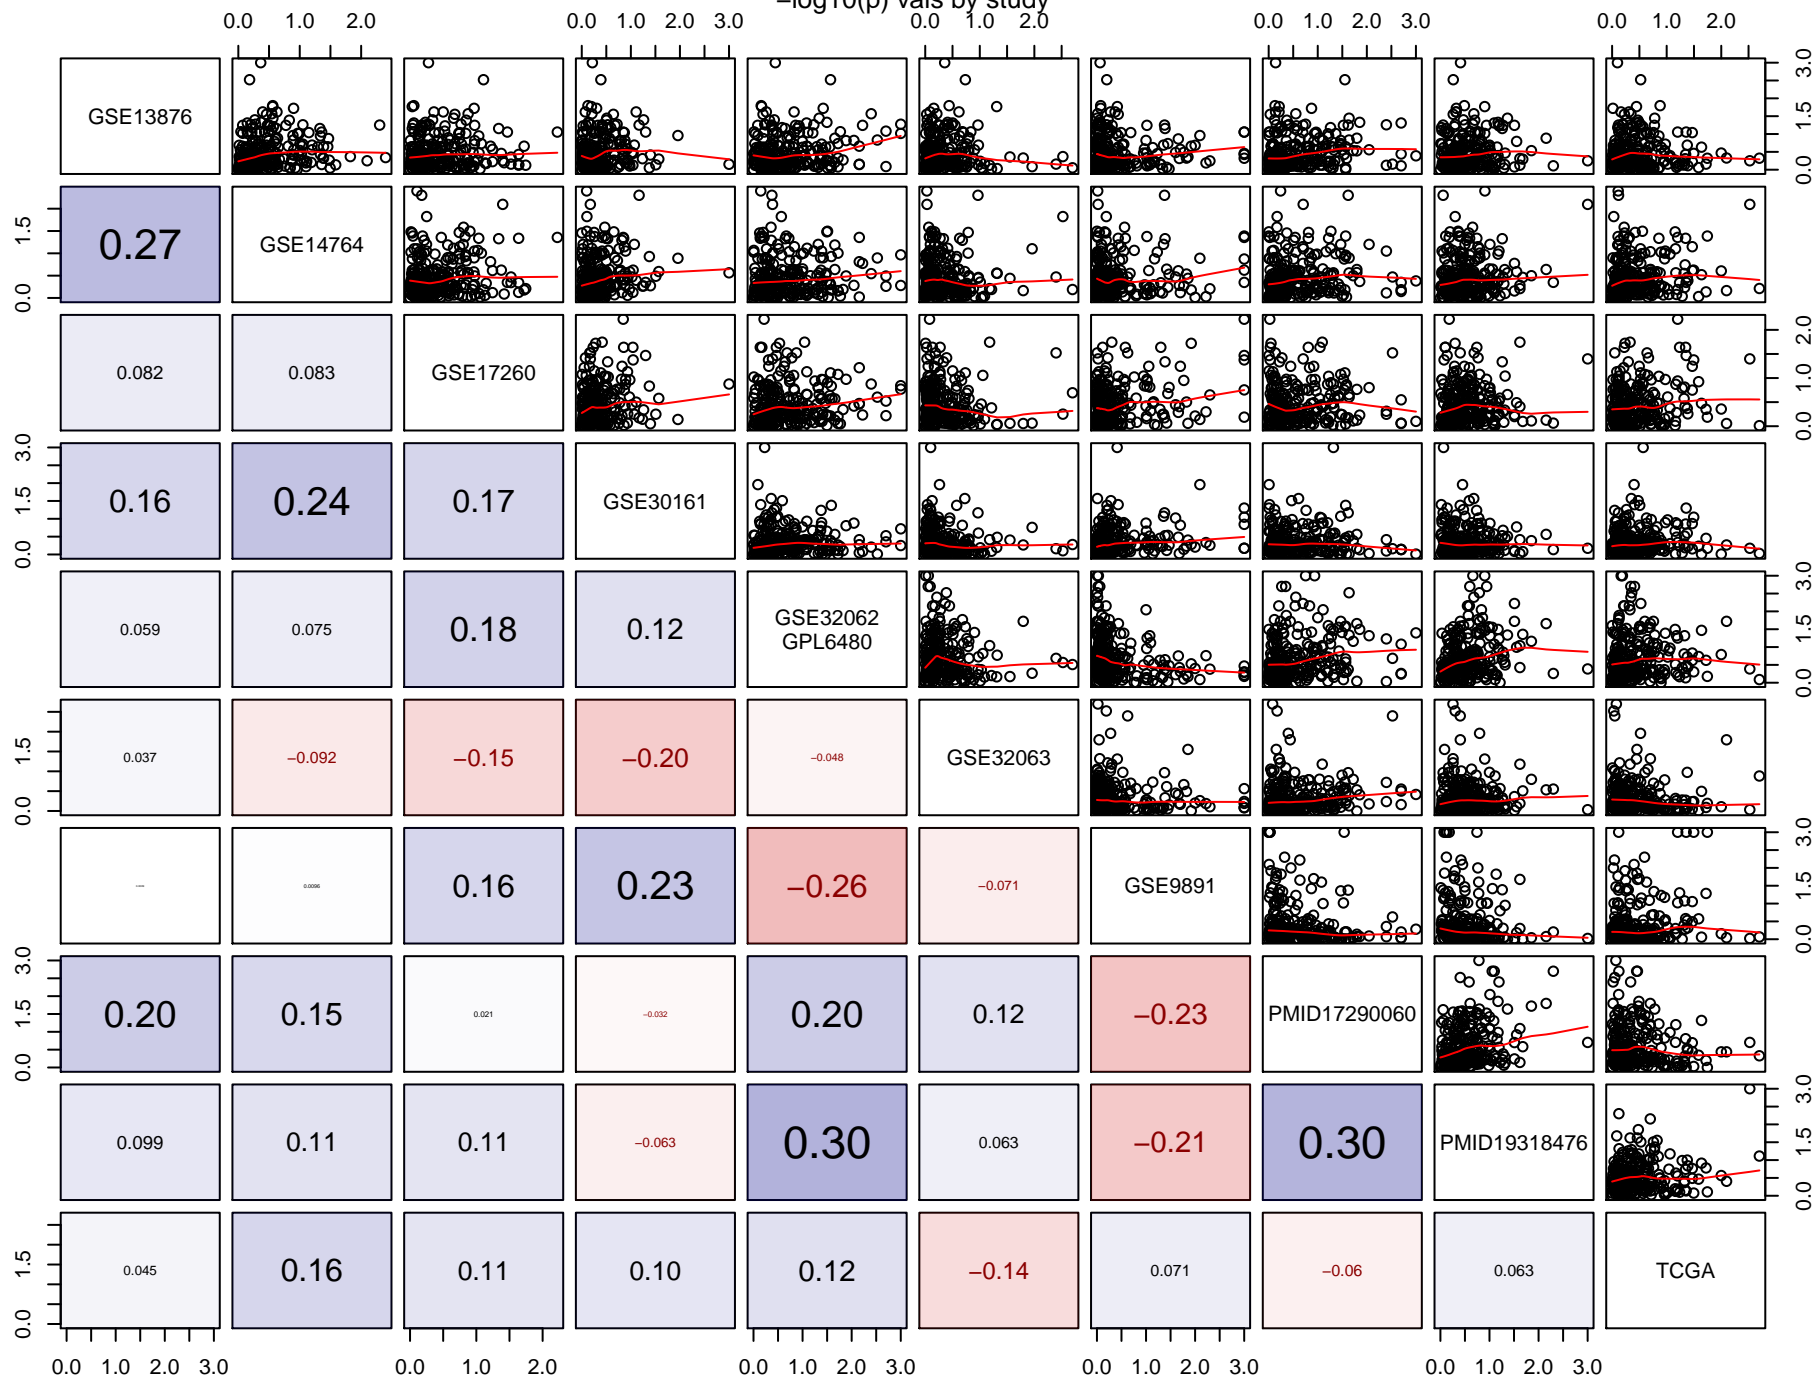

# SPIA.pComb analysis

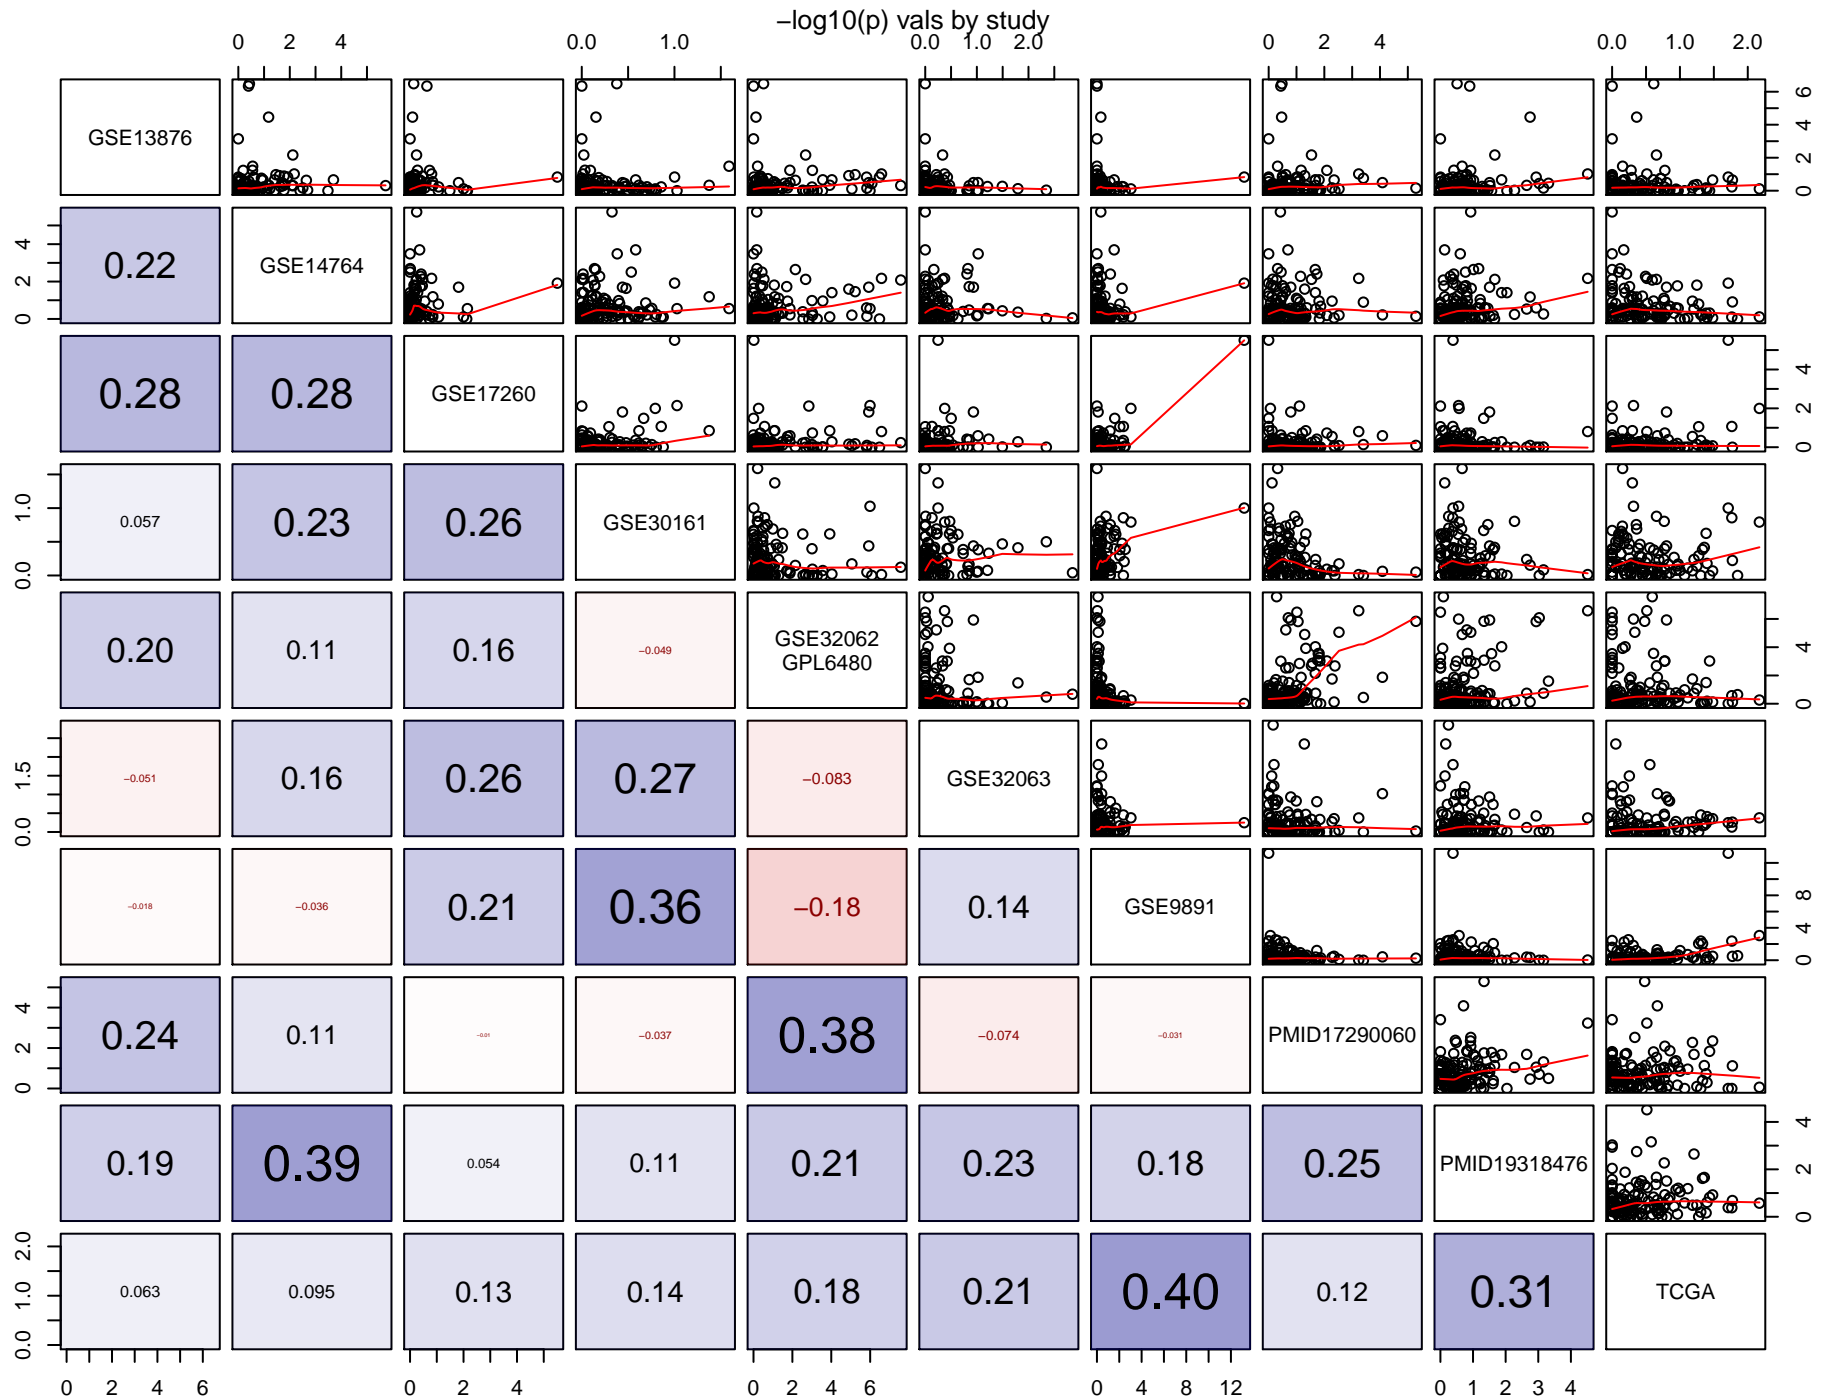

# ROTPe\_cutoff.pComb analysis

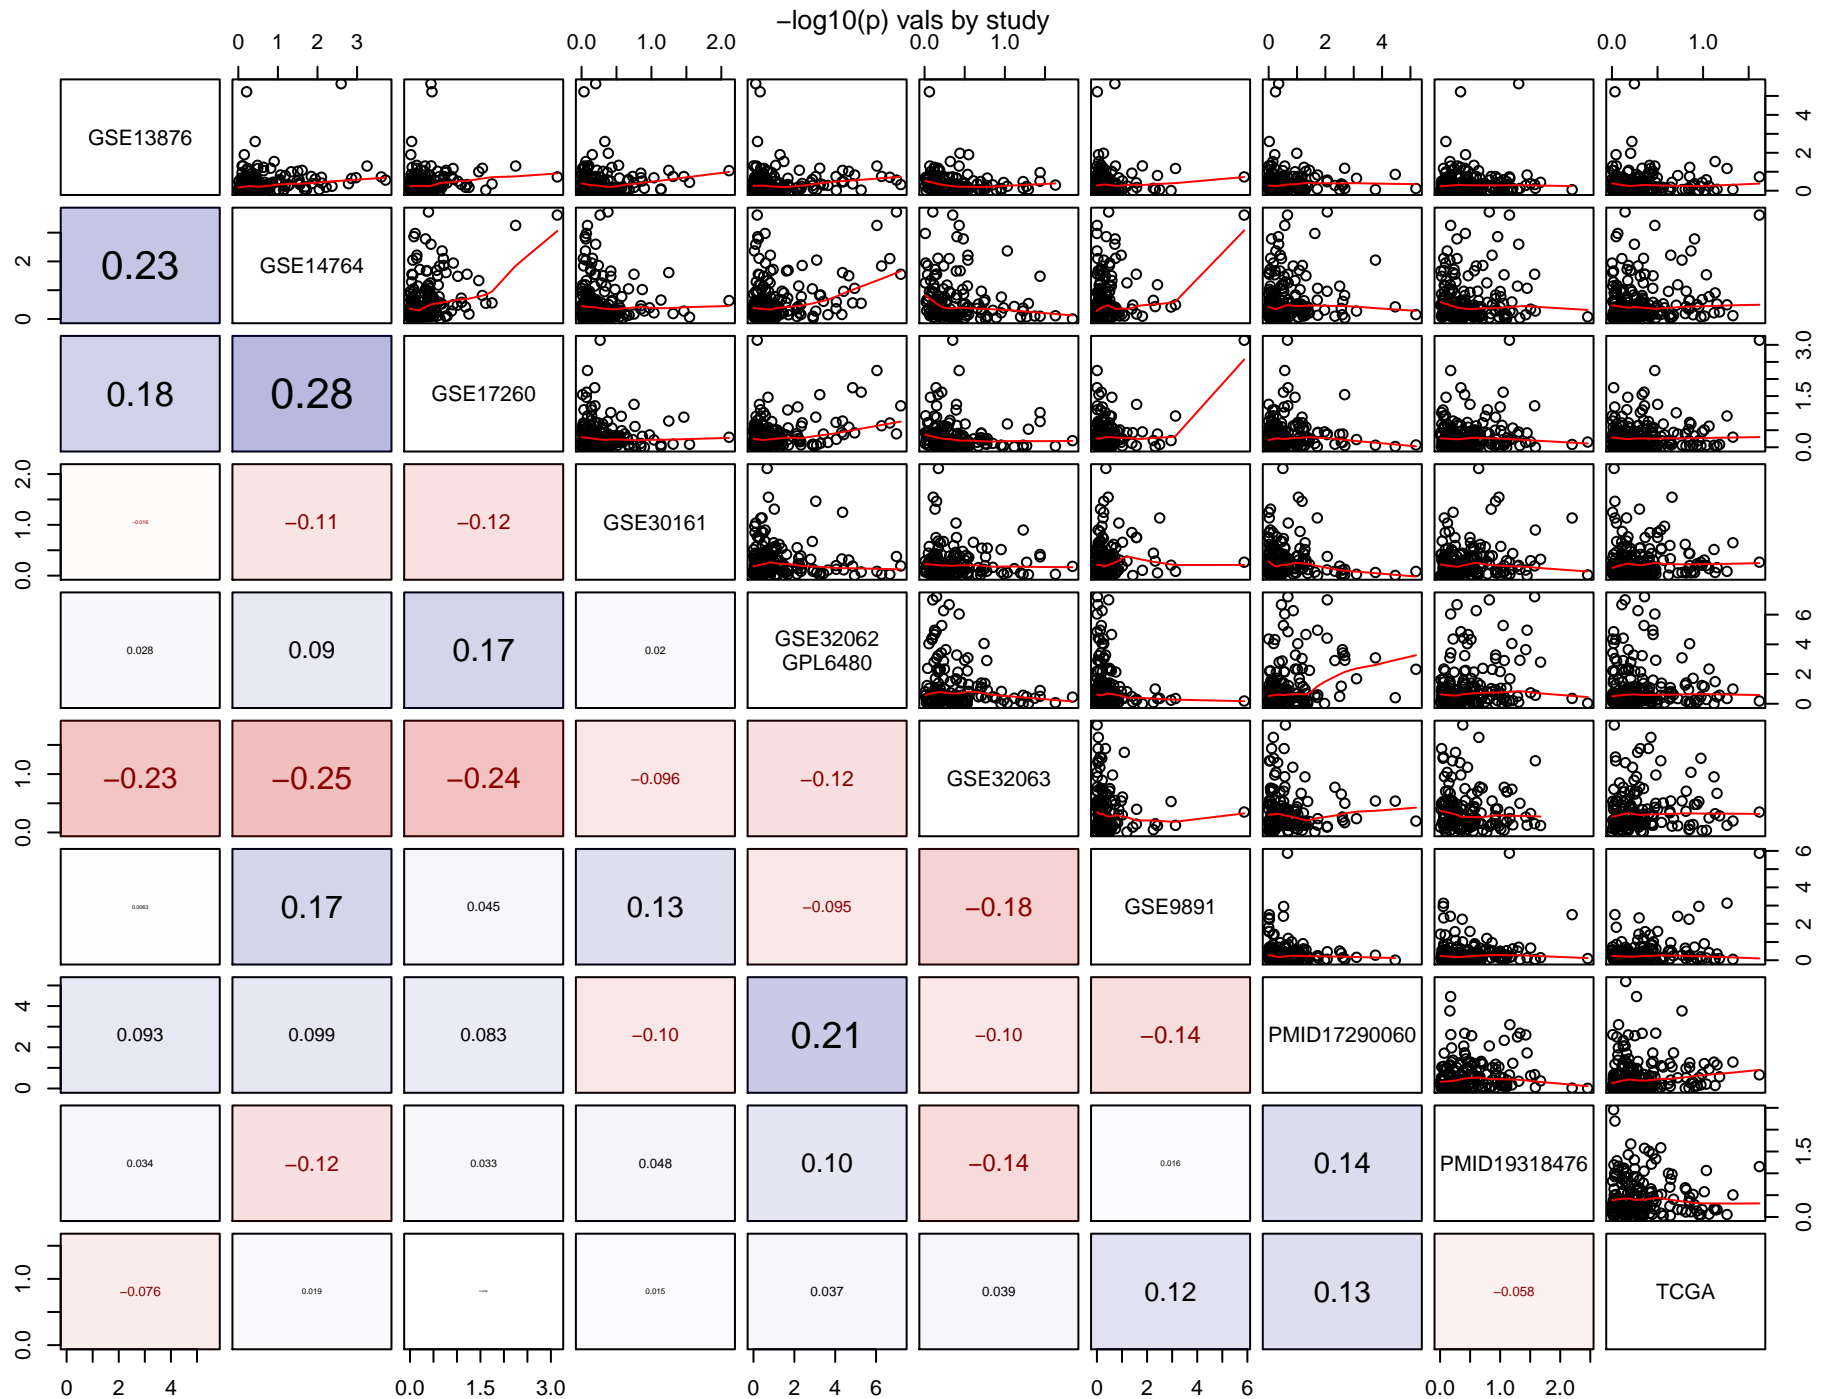

# ROTpe\_noCut.pPert analysis

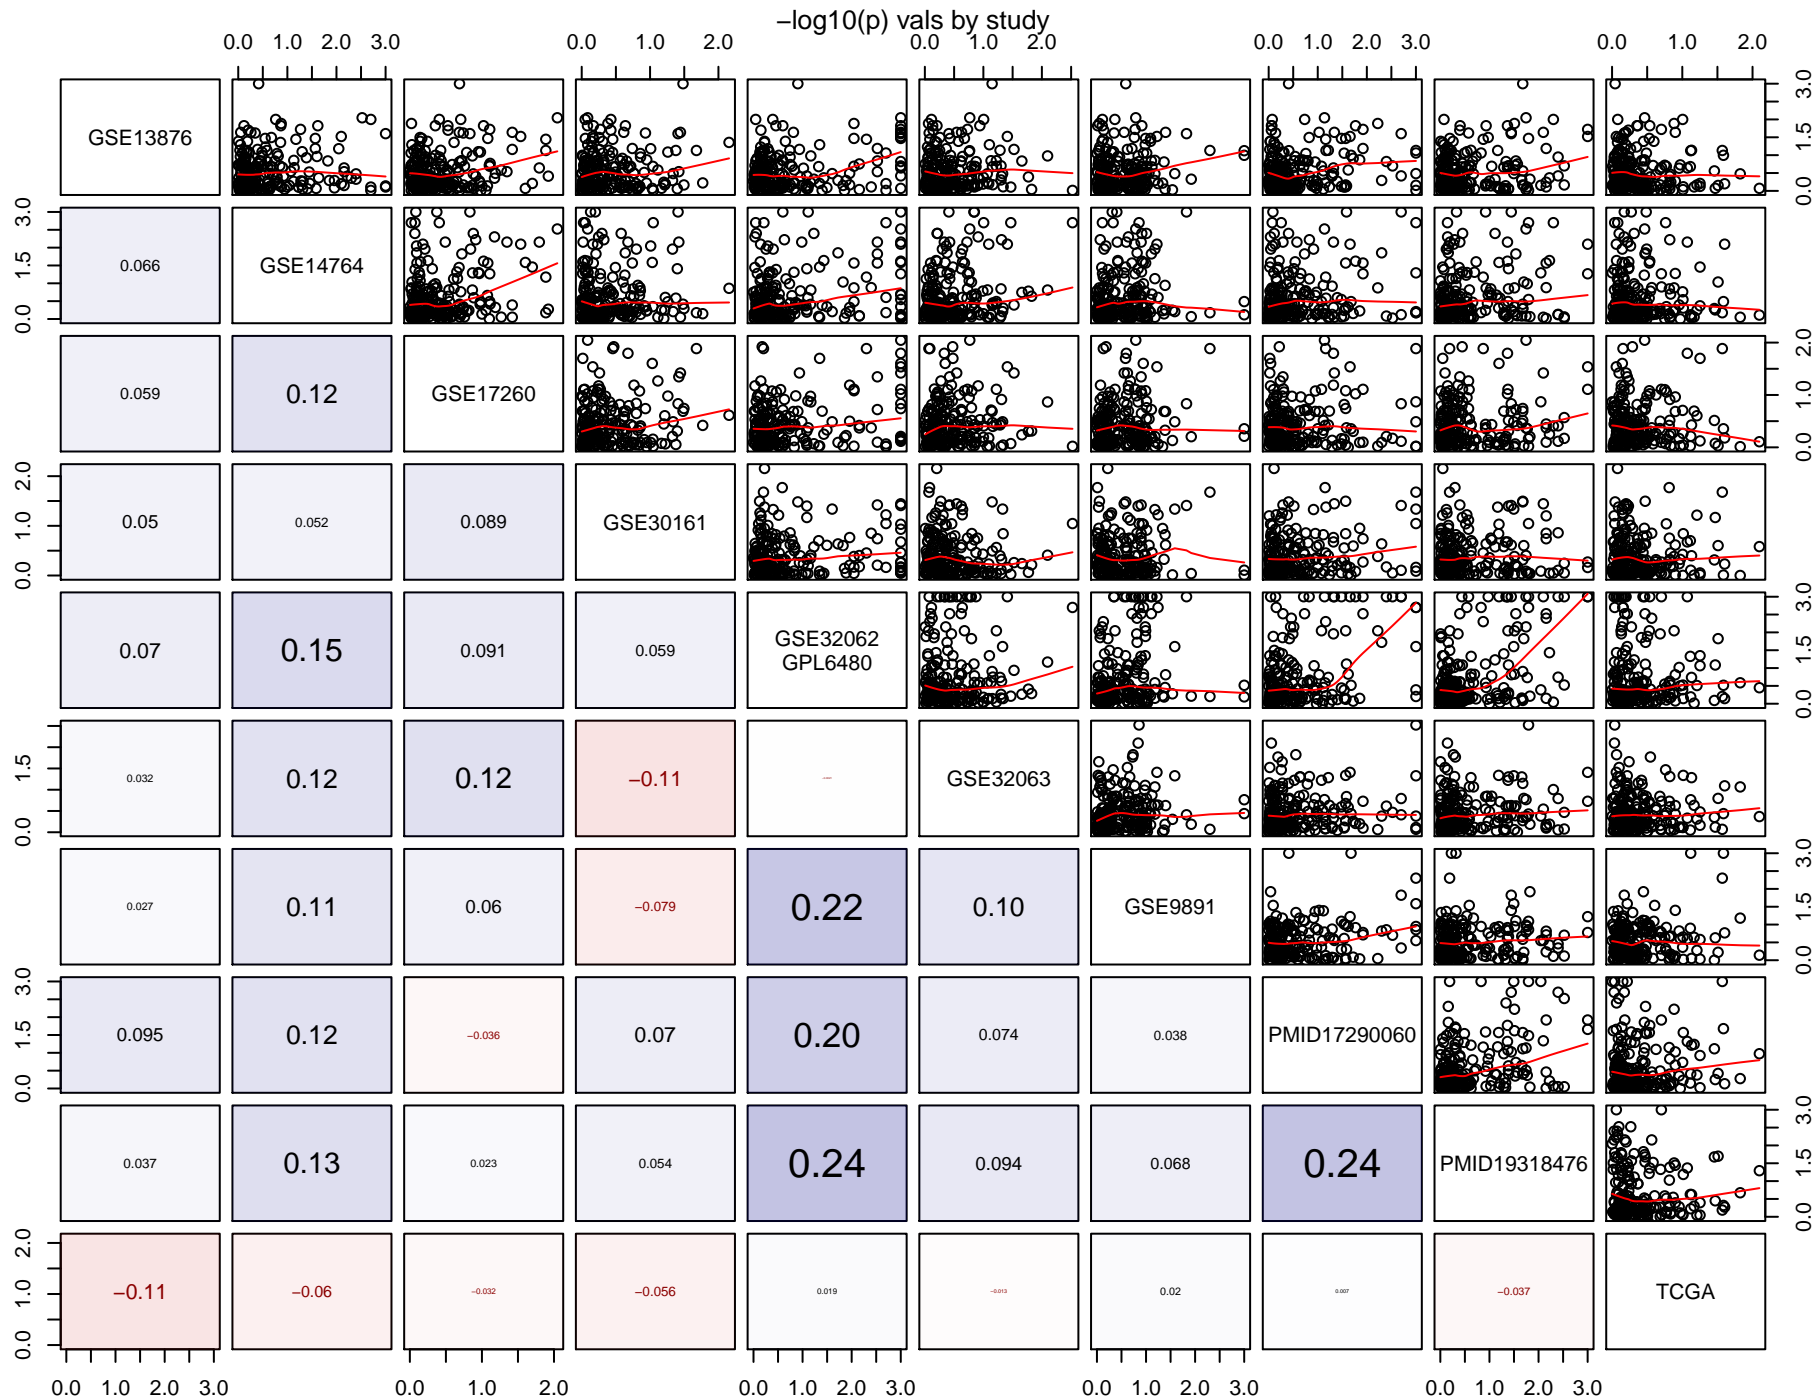

# PathNet.pPathNet analysis

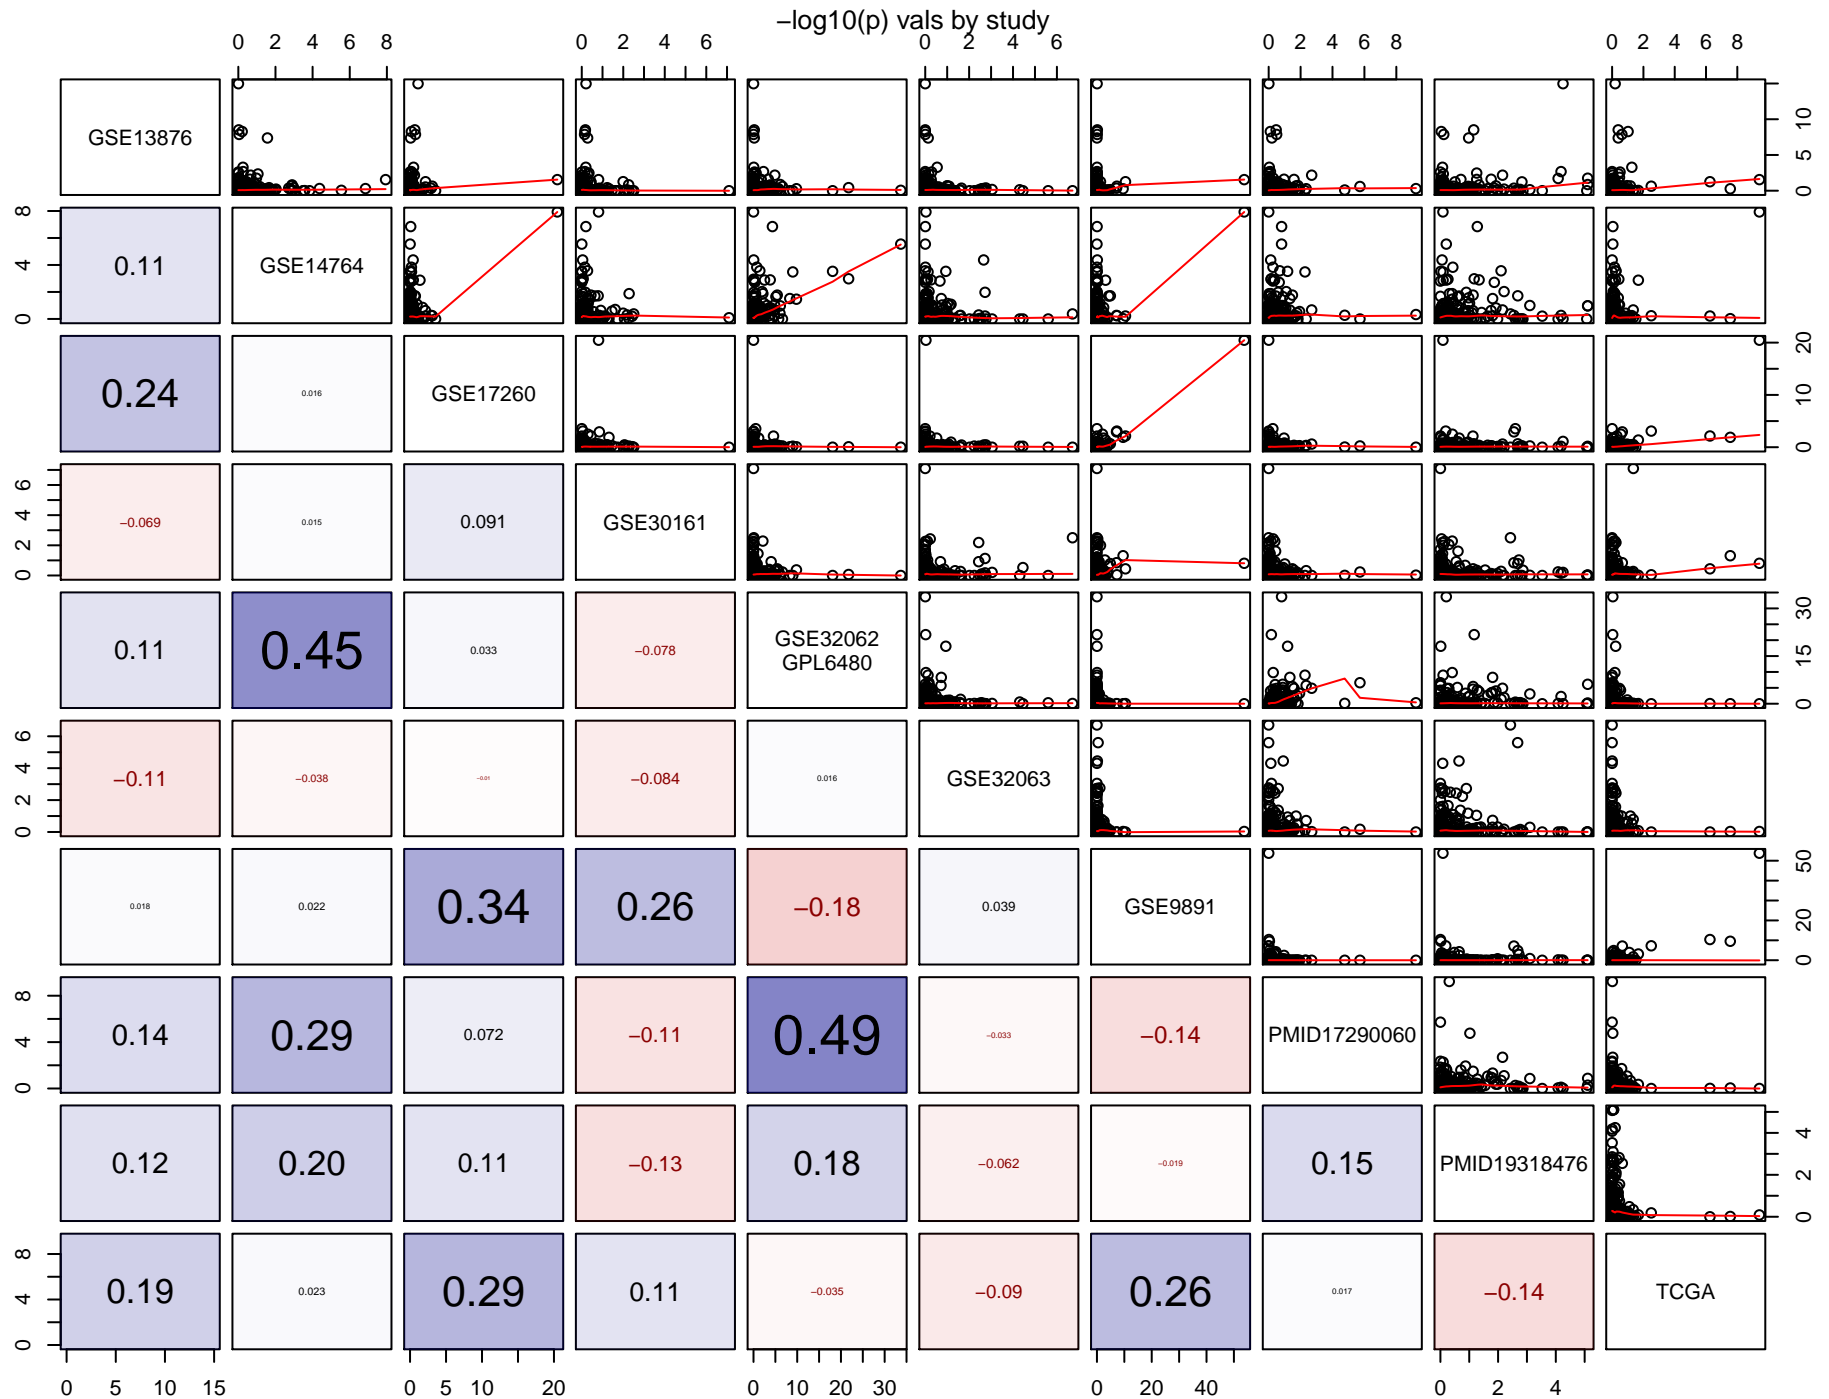



# NEA.pZ analysis

-log<sub>10</sub>(p) vals by study

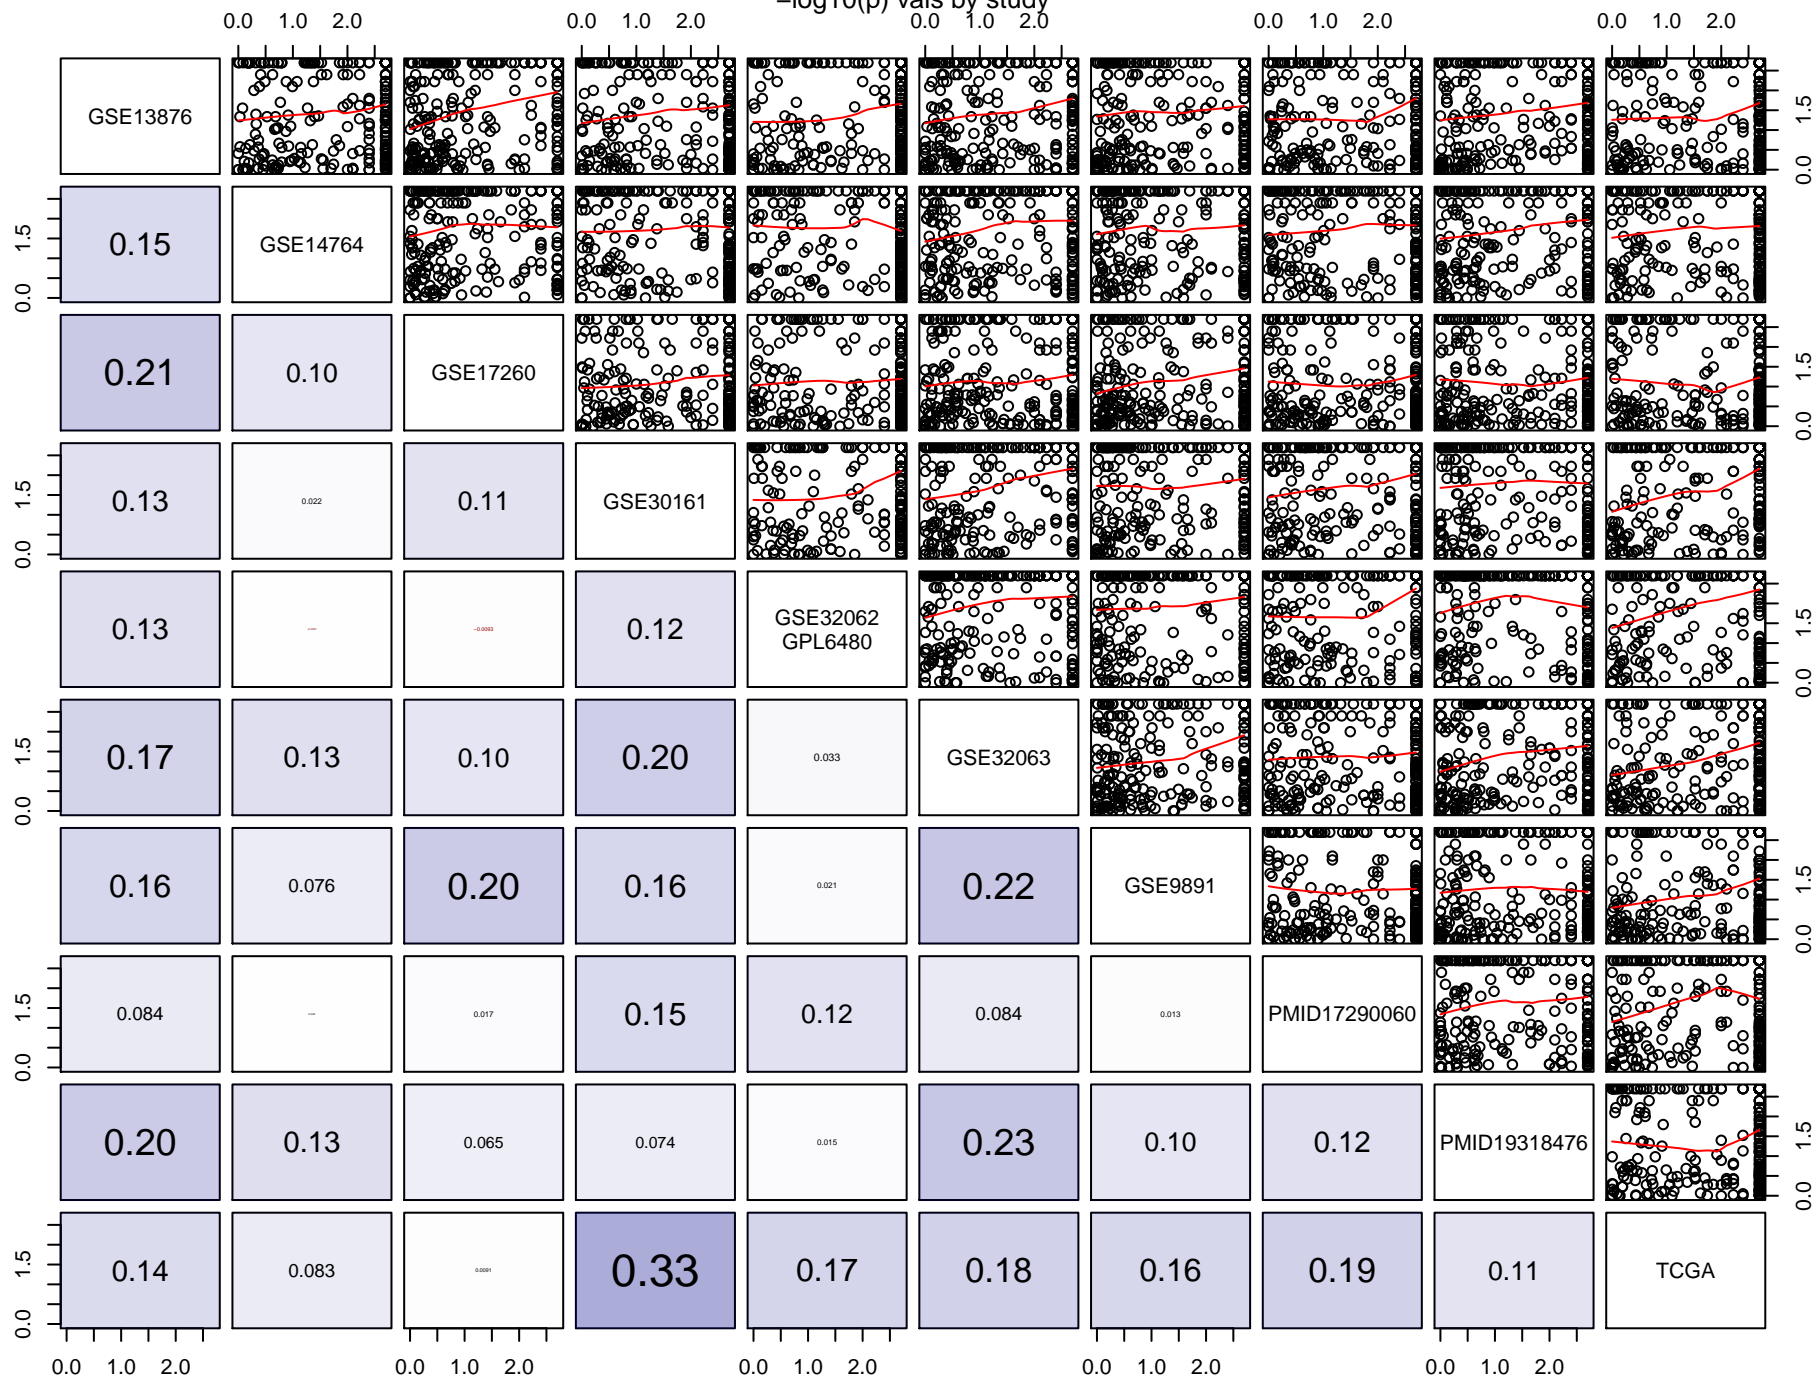

## CePa\_ORA.pComb analysis

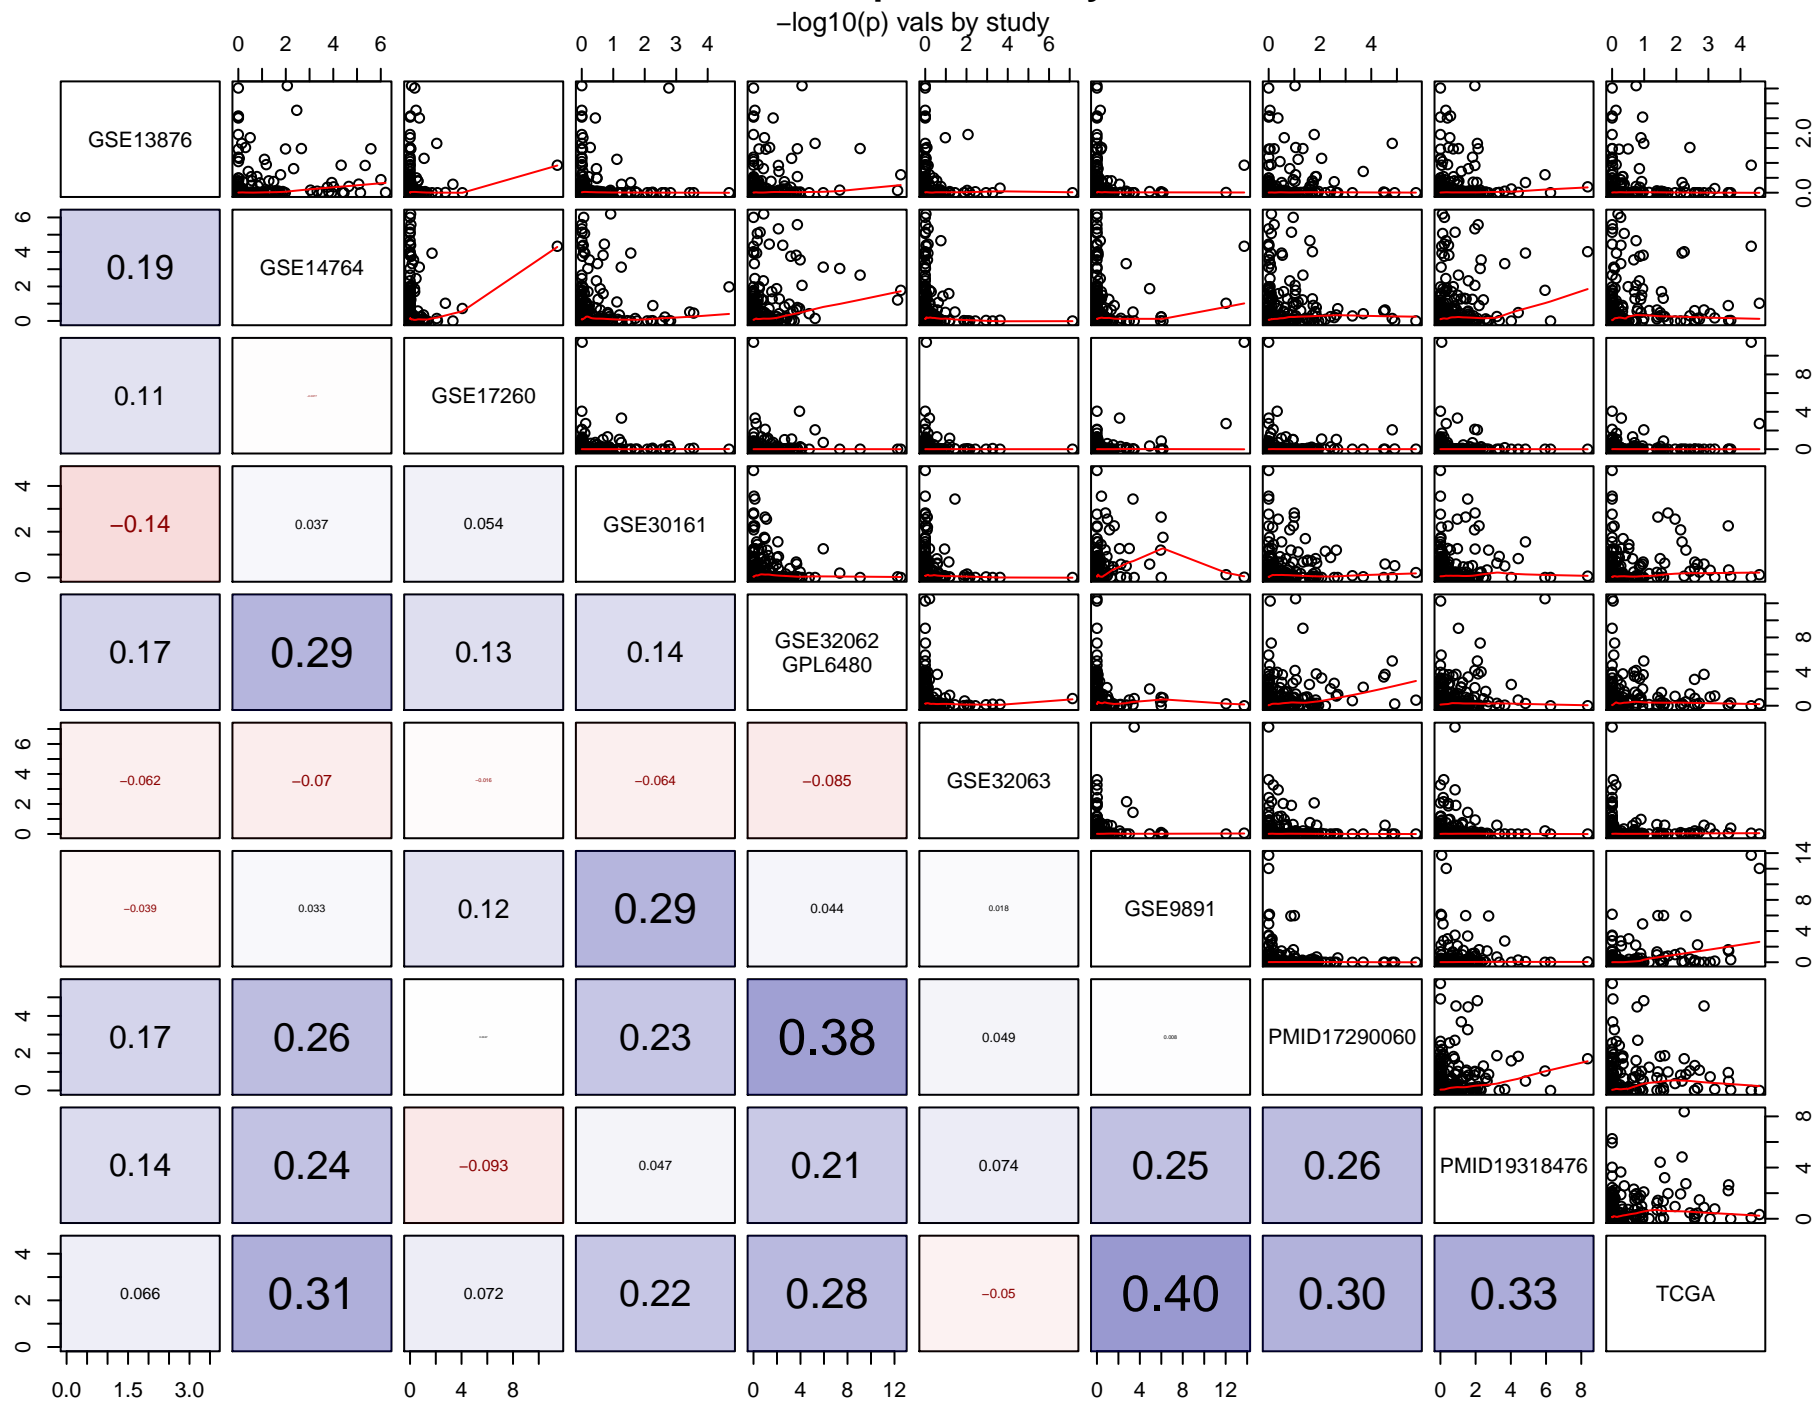



-log10(p) vals by study

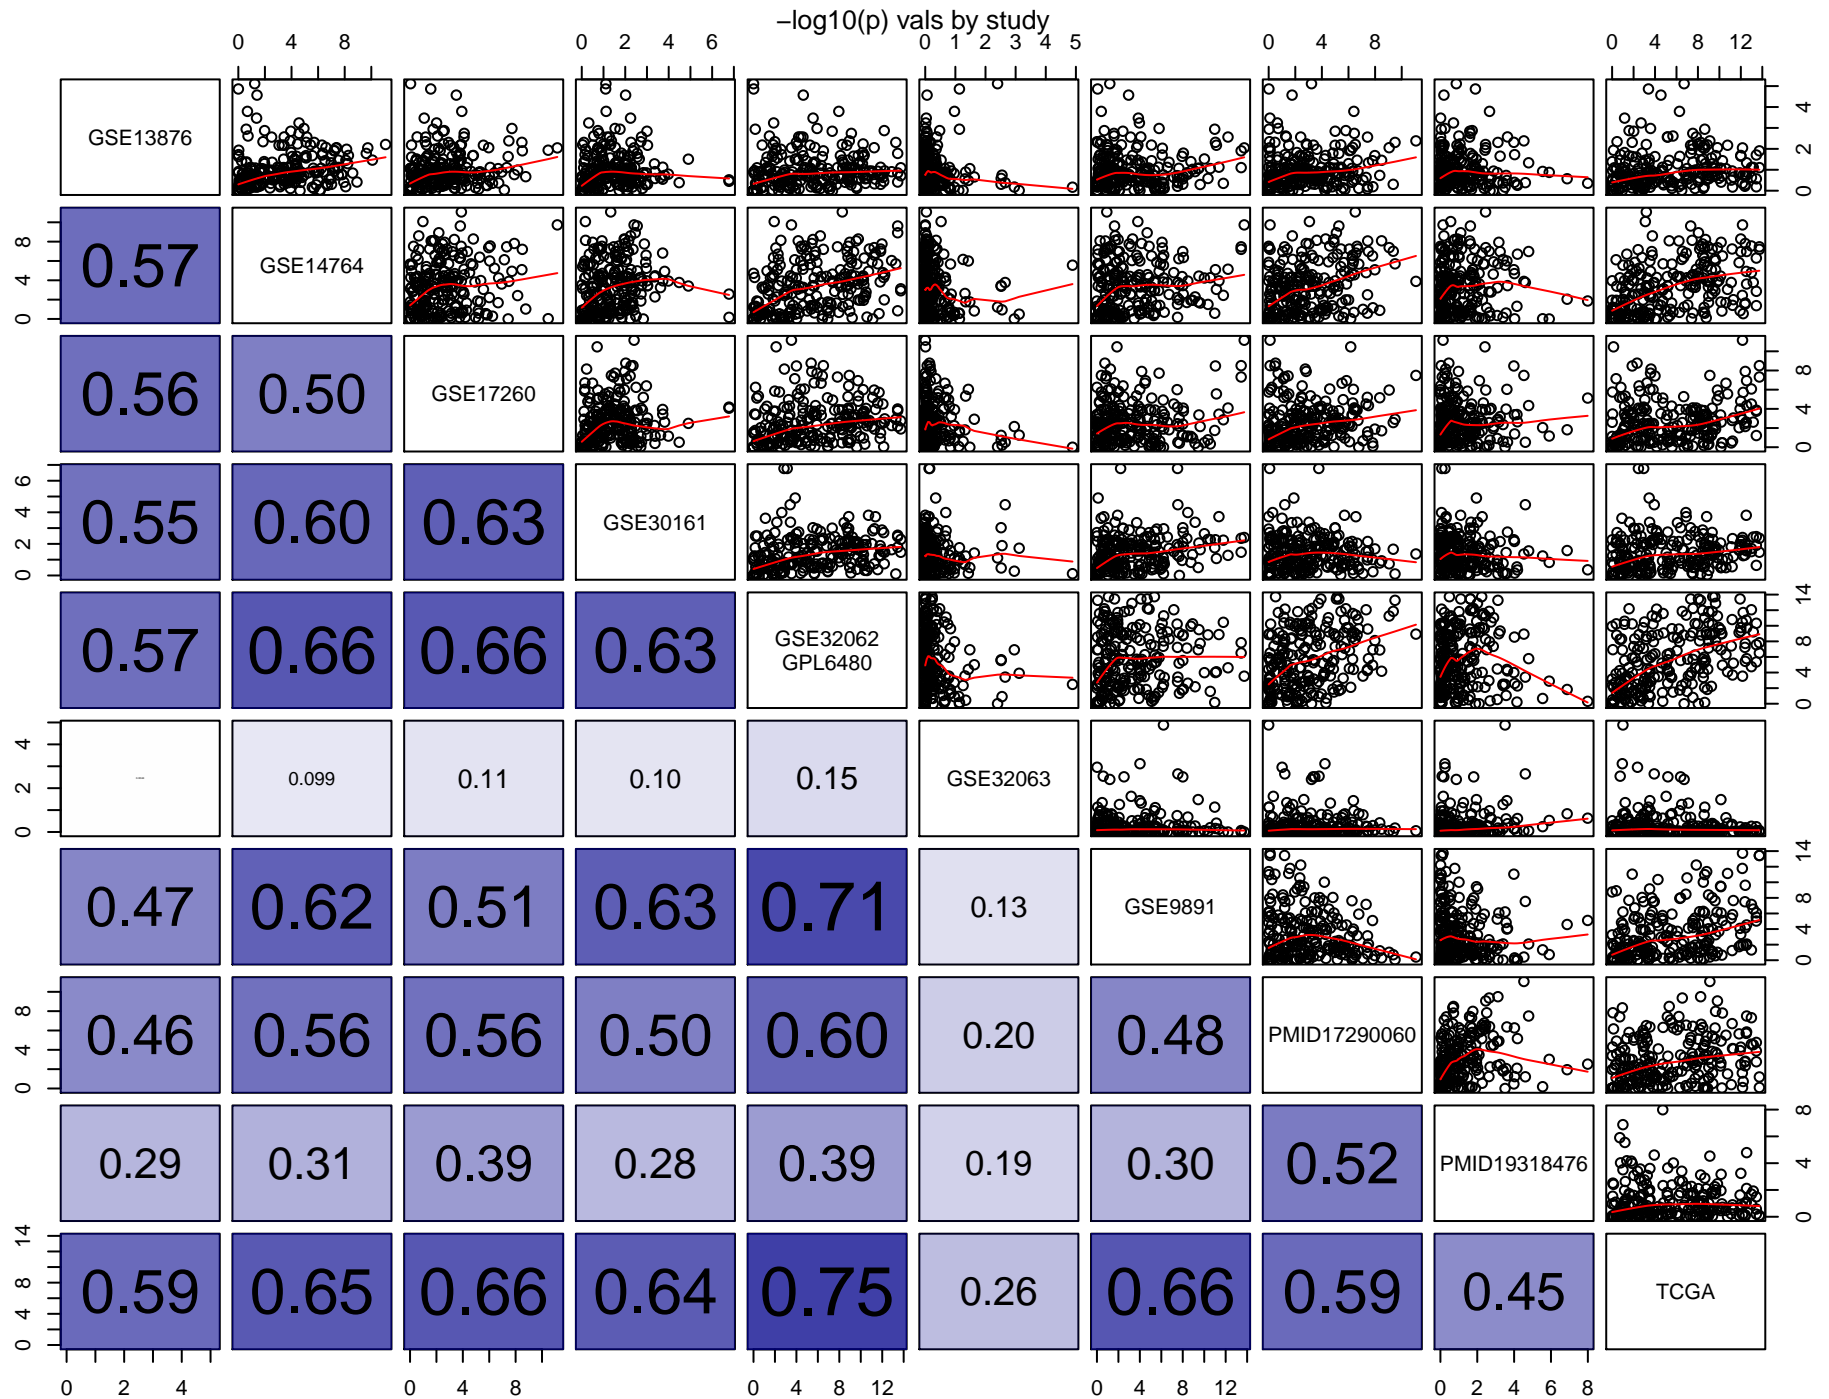

DEgraph\_signed.pT2graph analysis

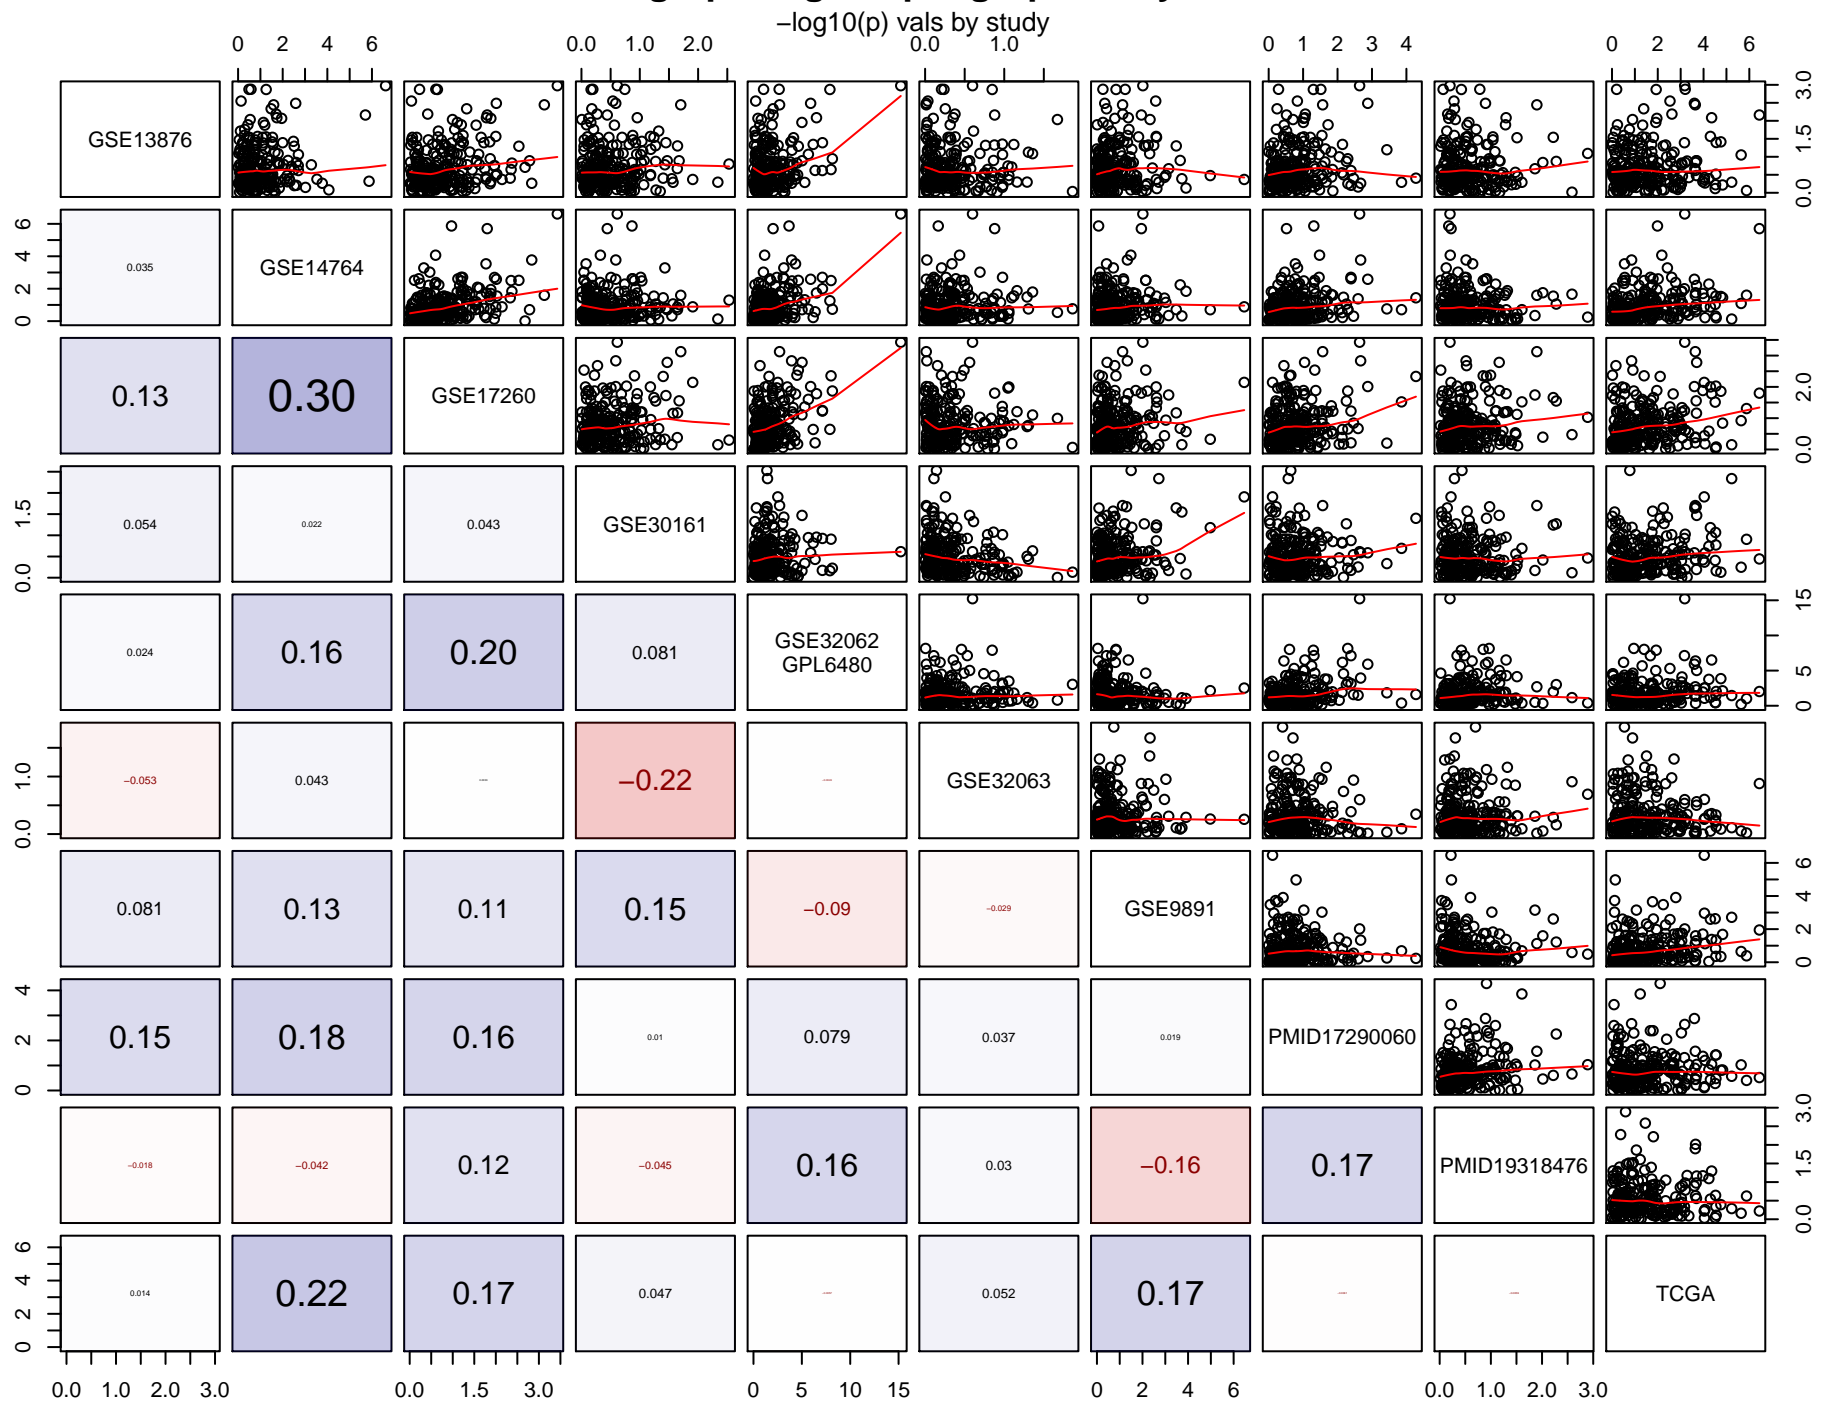

# DEgraph\_unsigned.pT2graph analysis

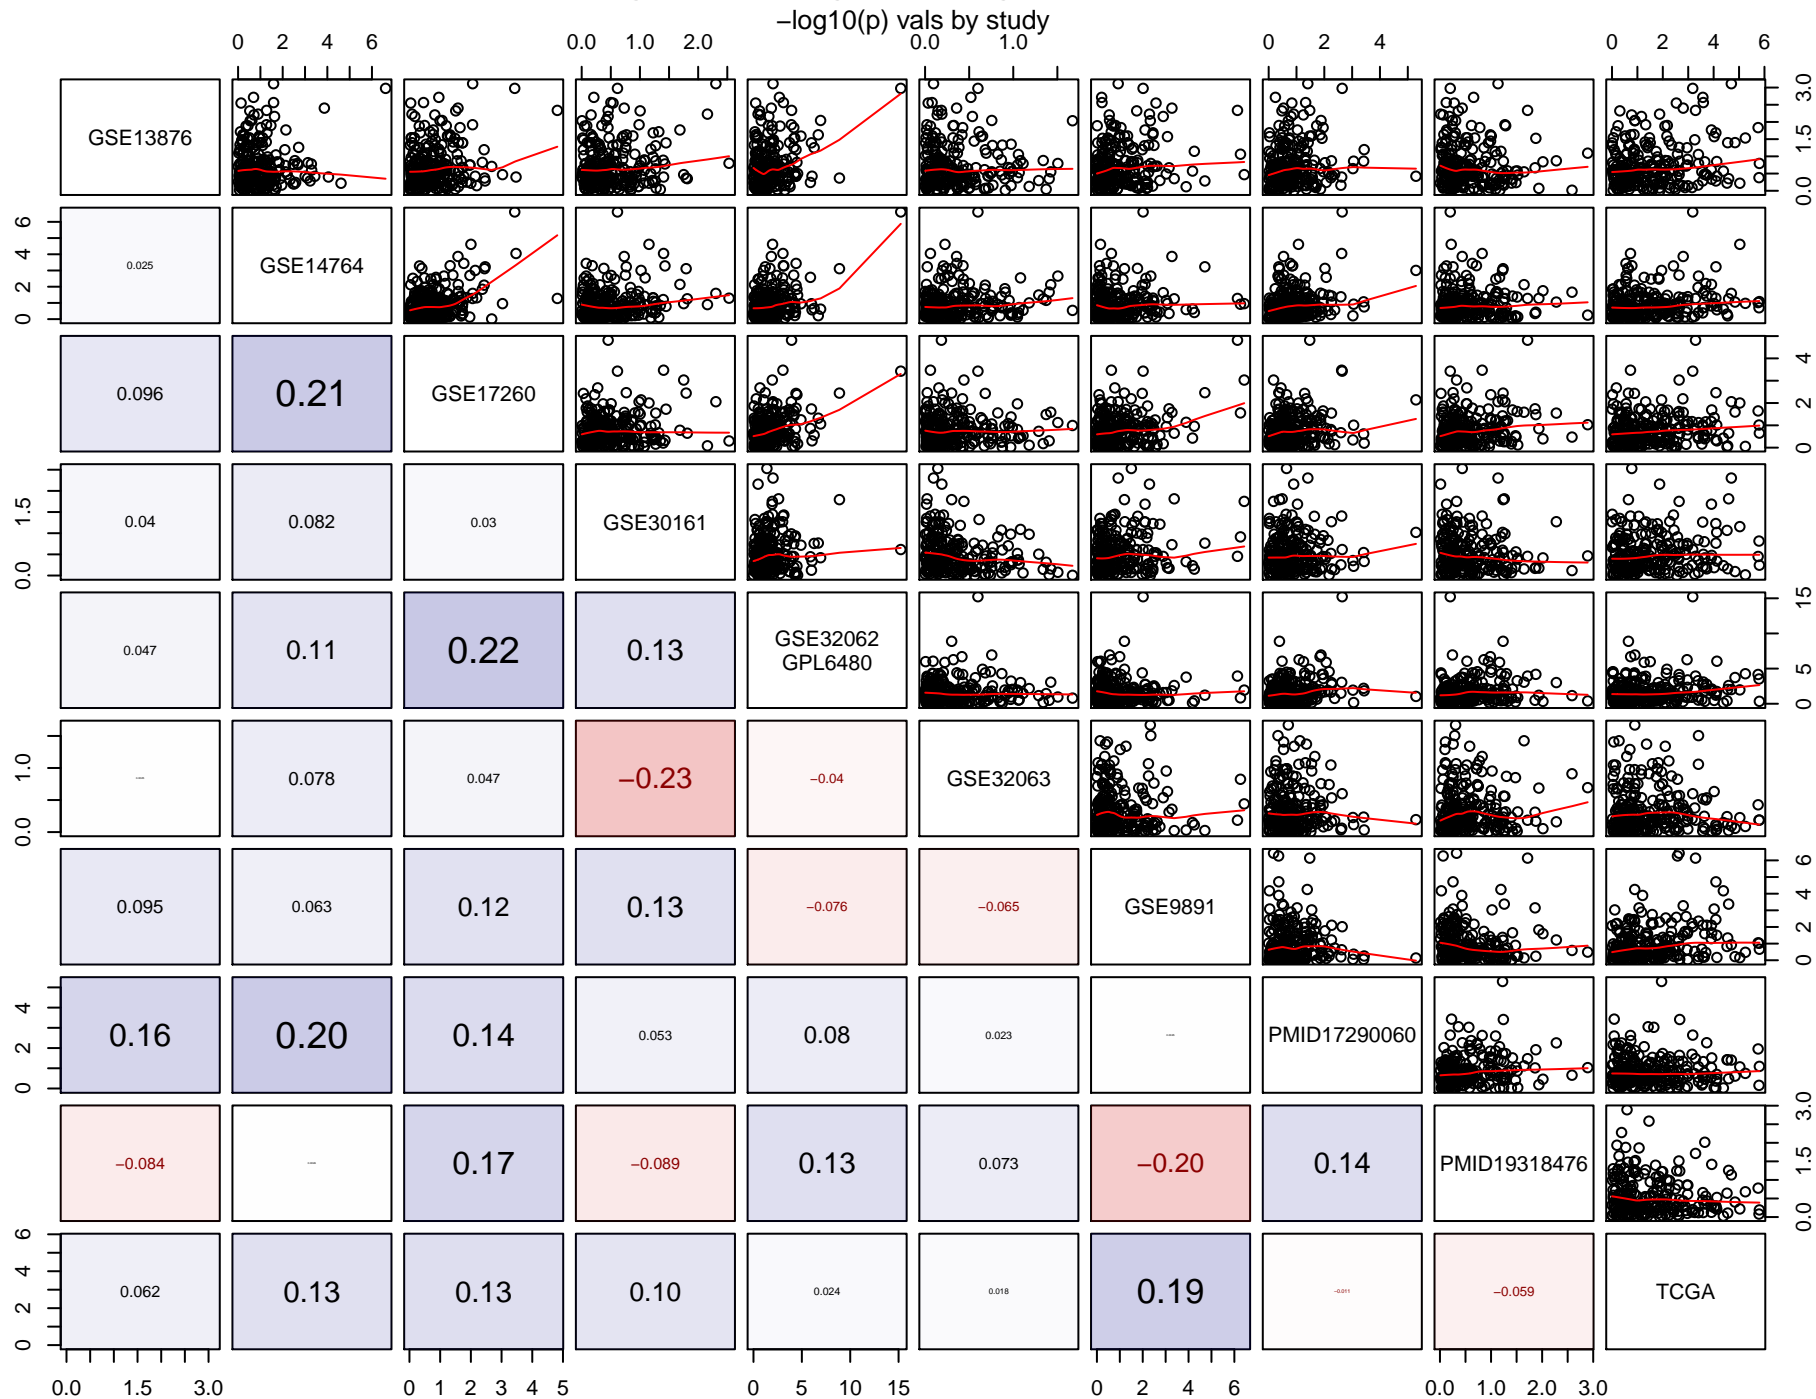

Supplement: Supplementary file 2 [file supp.xStudyPairs.pdf]
